# Supplementary material for: FedChain: Chained Algorithms for Near-Optimal Communication Cost in Federated Learning
Source: arXiv:2108.06869 source file (2023-04-16)
Supplement: Supplementary file 1 [file convexproofs.tex]

%!TEX root = ./main.tex
\section{Proofs under general convexity}
\subsection{Proofs for tail algorithms}
\subsubsection{\mbsgd}
\begin{proposition}
    \label{prop:convex-sgd}
    Suppose we run \mbsgd \pcref{algo:mbsgd} under $\beta$-smoothness assumption \pcref{asm:smooth}, bounded variance assumption \pcref{asm:uniform_variance}, and bounded initial distance/suboptimality \pcref{asm:distance}/\pcref{asm:subopt}.  Then if we set $\eta = \min \{\frac{1}{\beta}, (\frac{2 \Delta N K}{\beta \sigma^2 R})^{1/2} \}$ and return a uniformly sampled iterate from the $\x{r}$'s denoted as $\hat{x}$,
    \begin{align}
        \E \|\nabla F(\hat{x})\|^2 \leq \frac{2 \beta \Delta}{R} + \frac{2 \beta \sigma D }{\sqrt{N K R}}
    \end{align}
    and
    \begin{align}
        \E \|\hat{x} - x^*\|^2 \leq 3 D^2
    \end{align}
\end{proposition}
\begin{proof}
    By smoothness \pcref{asm:smooth}, we have that 
    \begin{align}
        F(\x{r + 1}) - F(\x{r}) \leq -\eta \langle \nabla F(\x{r}), \frac{1}{NK} \sum_{i=1}^N \sum_{k=0}^{K-1} g_{i,k}^{(r)} \rangle + \frac{\beta \eta^2}{2} \|\frac{1}{NK} \sum_{i=1}^N \sum_{k=0}^{K-1} g_{i,k}^{(r)}\|^2
    \end{align}
    Taking expectation conditioned up to $r$ and using \cref{asm:uniform_variance} and \cref{lemma:minibatchvariance}.
    \begin{align}
        \E_r F(\x{r + 1}) - F(\x{r}) \leq -(\eta - \frac{\beta \eta^2}{2}) \|\nabla F(\x{r})\|^2 + \frac{\beta \sigma^2 \eta^2}{2 N K}
    \end{align}
    If $\eta \leq \frac{1}{\beta}$,
    \begin{align}
        \label{eq:convex-unroll-sgd}
        \E_r F(\x{r + 1}) - F(\x{r}) \leq -\frac{\eta}{2} \|\nabla F(\x{r})\|^2 + \frac{\beta \sigma^2 \eta^2}{2 N K}
    \end{align}
    Taking full expectation and rearranging,
    \begin{align}
        \frac{1}{2} \E \|\nabla F(\x{r})\|^2 \leq \frac{\E F(\x{r+1}) - \E F(\x{r})}{\eta} + \frac{\beta \sigma^2 \eta}{2 N K}
    \end{align}
    Summing both sides over $r$ and averaging,
    \begin{align}
        \frac{1}{2} \frac{1}{R} \sum_{r = 0}^{R-1} \E \|\nabla F(\x{r})\|^2 \leq \frac{\E F(\x{0}) - \E F(\x{R})}{\eta R} + \frac{\beta \sigma^2 \eta}{2 N K}
    \end{align}
    Letting $\hat{x}$ be a uniform sample from all the $\x{r}$'s, noting that $\E F(\x{0}) - \E F(\x{R}) \leq \Delta$, $\Delta \leq \beta D^2$, and choosing $\eta = \min \{\frac{1}{\beta}, (\frac{2 \Delta N K}{\beta \sigma^2 R})^{1/2} \}$
    \begin{align}
        \E \|\nabla F(\hat{x})\|^2 \leq \frac{2 \beta \Delta}{R} + \frac{2 \beta \sigma D }{\sqrt{N K R}}
    \end{align}
    Next observe that 
    \begin{align}
        \|x^{(r+1)} - x^*\|^2 = \|x^{(r)} - x^*\|^2 - 2 \eta \langle x^{(r)} - x^*, g_{i,k}^{(r)} - \nabla F(x^*) \rangle + \eta^2 \|g_{i,k}^{(r)} - \nabla F(x^*)\|^2
    \end{align}
    Taking expectation up to $r$ and using the smoothness gradient co-coercivity property,
    \begin{align}
        \E_r \|x^{(r+1)} - x^*\|^2 &\leq \|x^{(r)} - x^*\|^2 - \frac{2 \eta}{\beta} \| \nabla F(\x{r}) - \nabla F(x^*) \|^2+ \eta^2 \E_r \|g_{i,k}^{(r)} - \nabla F(x^*)\|^2 \\
        &\leq \|x^{(r)} - x^*\|^2- \frac{2 \eta}{\beta} \| \nabla F(\x{r}) - \nabla F(x^*) \|^2 + \eta^2 \| \nabla F(\x{r}) - \nabla F(x^*)\|^2 + \frac{\eta^2 \sigma^2}{NK}
    \end{align}
    And by the stepsize choice, we have that 
    \begin{align}
        \E \| \x{r+1} - x^*\|^2 \leq \E \|x^{(r)} - x^*\|^2 + \frac{2 D^2}{R} 
    \end{align}
    Which implies that 
    \begin{align}
        \E \| \hat{x} - x^*\|^2 \leq 3 D^2
    \end{align}
\end{proof}
\begin{proposition}
    \label{prop:appsgdconvex-func}
    Suppose $F$ is general convex \pcref{asm:convex}, $\beta$-smooth \pcref{asm:smooth}, and each client gradient variance is bounded as $\sigma^2$ \pcref{asm:uniform_variance}.  Then suppose we run \mbsgd \pcref{algo:mbsgd} on a modified loss in the setting of Theorem 1 of \cite{woodworth2020minibatch}
    \begin{align}
        f_\mu(x;z) = f(x;z) + \frac{\mu}{2} \|x - x^{(0)}\|^2
    \end{align}
    where $x^{(0)}$ is the initial iterate, and 
    \begin{align}
        \mu \geq \frac{16 \beta}{R^2}\log^2(e^2 + R^2) \qquad \mu \geq (\frac{ 144 \sigma^2 }{  D^2 N K R})^{1/2}
    \end{align}
    If we return the final iterate
    \begin{align}
        \hat{x} = x^{(R)}
    \end{align}
    Then we have the following guarantee:
    \begin{align}
        \E F(\hat{x}) - F(x^*) \leq \min \{ 130 \Delta, \frac{ 136 \beta D^2 }{R} \log (e^2 + R) \}+ \frac{12 \sigma D}{ \sqrt{N K R}}
    \end{align}
    and 
    \begin{align}
        \E \|\hat{x} - x^*\|^2 \leq 33 D^2
    \end{align}
    so long as $R \geq 192$ \footnote{We assume this constant lower bound for technical simplification, as in \citep{yuan2020federatedac}.}

\end{proposition}
\begin{proof}
    Let $F_\mu(x) = F(x) + \frac{\mu}{2} \|x - x^{(0)}\|^2$, where $x^{(0)}$ is the initial iterate.   Also let $x^*_\mu = \argmin_x F_\mu(x)$ and $\Delta_{\mu} := \E [F_\mu(x^{(0)}) - F_\mu(x^*_\mu)]$. 
    
    We know that running \cref{algo:mbsgd} on $F_\mu$ in the setting of \cite{woodworth2020minibatch} (noting that $F_\mu$ is $\beta + \mu$-smooth), 
    we can achieve convergence rates where $\kappa' = \frac{\beta + \mu}{\mu}$
    \begin{align}
        \E F_\mu(x^{(R)}) - F_\mu(x^*_\mu)  \leq 128 \kappa \Delta_\mu \exp(-\frac{R}{8 \kappa'}) + \frac{72 \sigma^2}{\mu N K R}
    \end{align}
    and
    \begin{align}
        \E F_\mu(x^{(R)}) - F_\mu(x^*_\mu)  \leq 128 \beta D^2 \exp(-\frac{R}{8 \kappa'}) + \frac{72 \sigma^2}{\mu N K R}
    \end{align}
    From the proof of \cref{lemma:convsmooth} \cref{eq:smooth-func-bound} and \cref{lemma:suboptupper} we have that with the settings for $\mu$ and requiring $R \geq 8 \kappa' \log(\kappa')$
    \begin{align}
        \E F(\hat{x}) - F(x^*) &\leq 130\Delta_\mu + \frac{12 \sigma D}{\sqrt{NKR}}
    \end{align}
    Now observe that 
    \begin{align}
        F_\mu(x_\mu^*) = F(x_\mu^*) + \frac{\mu}{2} \|x_\mu^* - x^{(0)}\|^2 \leq F(x^*) + \frac{\mu}{2} \|x^* - x^{(0)}\|^2
    \end{align}
    So 
    \begin{align}
        F(\hat{x}) - F(x^*) = F_\mu(\hat{x}) - F(x^*) -\frac{\mu}{2}\|\hat{x} - x^{(0)}\|^2 \leq F_\mu(\hat{x}) - F_\mu(x^*_\mu) + \frac{\mu}{2} D^2
    \end{align}
    So we have that 
    \begin{align}
        \E F(\hat{x}) - F(x^*) \leq 128 \beta D^2 \exp(-\frac{R}{8 \kappa'}) + \frac{72 \sigma^2}{\mu N K R} + \frac{\mu}{2} D^2
    \end{align}
    Now recall the following settings for $\mu$:
    \begin{align}
        \mu \geq \frac{16 \beta}{R}\log(e^2 + R) \qquad \mu \geq (\frac{ 144 \sigma^2 }{  D^2 N K R})^{1/2}
    \end{align}
    requiring $R \geq 192$,
    \begin{align}
        \E F(\hat{x}) - F(x^*) \leq \frac{ 136 \beta D^2 }{R} \log (e^2 + R) + \frac{12 \sigma D}{\sqrt{NKR}}
    \end{align}
    To finish the first guarantee, observe that with the choice of $\mu \geq \frac{16 \beta}{R^2}\log(e^2 + R)$, $R \geq 8 \kappa' \log \kappa'$ is always satisfied, and apply $\Delta \leq \beta D^2$ to the second term.  For the second guarantee, follow the proof of \cref{prop:appasgconvex}.
\end{proof}
\begin{proposition}
    \label{prop:sampled_fedavg}
    Suppose we run \cref{algo:fedavg} with $\eta = \frac{1}{\beta}$ on the regularized objective
    \begin{align}
        F_\mu(x) = F(x) + \frac{\mu}{2} \|x^{(0)} - x\|^2
    \end{align}
    Then we have 
    \begin{align}
        \E F(x^{(R)}) - F(x^*) \leq \tilde{\mathcal{O}}(\frac{\beta D^2}{\sqrt{K} R} + \frac{\sigma D}{K^{1/4}} + \zeta D )
    \end{align}
    and 
    \begin{align}
        \E\|x^{(R)} - x^*\|^2 \leq \tilde{\mathcal{O}}(D^2)
    \end{align}
\end{proposition}
\begin{proof}
    We know that running \cref{algo:fedavg} with $\eta = \frac{1}{\beta}$ gives (from \cref{thm:fedavgstrong})
    \begin{align}
        \E F_\mu(x^{(R)}) - F_\mu(x^*_\mu) \leq  \Delta_\mu \exp(-\frac{R \sqrt{K}}{\frac{\beta + \mu}{\mu}})+ \frac{\zeta^2}{2 \mu} + \frac{\sigma^2}{2\mu\sqrt{K}}
    \end{align}
    We have that from a proof very similar to Proposition E.7 in \citep{yuan2020federatedac}
    \begin{align}
        \E F(x^{(R)}) - F(x^*) \leq \E F_\mu(x^{(R)}) - F_\mu(x^*_\mu) + \frac{\mu}{2} D^2
    \end{align}
    So we have by \cref{lemma:suboptupper},
    \begin{align}
        \E F(x^{(R)}) - F(x^*) \leq \Delta \exp(-\frac{R \sqrt{K}}{\frac{\beta + \mu}{\mu}})+ \frac{\zeta^2}{2 \mu} + \frac{\sigma^2}{2\mu\sqrt{K}} + \frac{\mu}{2} D^2
    \end{align}
    Then if we choose $\mu \geq \Theta(\frac{\beta}{\sqrt{K} R} \log(e^2 + \sqrt{K} R))$, $\mu \geq \Theta(\frac{\zeta}{D})$, and $\mu \geq \Theta(\frac{\sigma}{D K^{1/4}})$,
    \begin{align}
        \E F(x^{(R)}) - F(x^*) \leq \tilde{\mathcal{O}}(\frac{\beta D^2}{\sqrt{K} R} + \frac{\sigma D}{K^{1/4}} + \zeta D )
    \end{align}

    Now we show the distance bound.  Recall that 
    \begin{align}
        \E F_\mu(x^{(R)}) - F_\mu(x^*_\mu) \leq  \Delta_\mu \exp(-\frac{R \sqrt{K}}{\frac{\beta + \mu}{\mu}})+ \frac{\zeta^2}{2 \mu} + \frac{\sigma^2}{2\mu\sqrt{K}}
    \end{align}
    By smoothness, strong convexity of $F_\mu$, and the choice of $\mu$, we have that
    \begin{align}
        \E\|x^{(R)} - x^*_\mu\|^2 \leq \tilde{\mathcal{O}}(D^2)
    \end{align}
    So,
    \begin{align}
        \E\|x^{(R)} - x^*\|^2 \leq 3\E\|x^{(R)} - x^*_\mu\|^2 + 3\E\|x^{(0)} - x^*_\mu\|^2 + 3\E\|x^* - x^{(0)}\|^2\leq \tilde{\mathcal{O}}(D^2)
    \end{align}
    Where the last inequality follows because 
    \begin{align}
        F(x^*_\mu) + \frac{\mu}{2}\|x^{(0)} - x^*_\mu\|^2 \leq F(x^*) + \frac{\mu}{2} \|x^{(0)} - x^*\|^2
    \end{align}
\end{proof}
\subsubsection{Sampled \lsgd $\to$ \mbsgd}
\begin{proof}
    By running \lsgd in the setting of \cref{prop:sampled_fedavg} as $\ahead$ and \mbsgd in the setting of \cref{prop:convex-sgd} as $\atail$ we have (because the per-iterate variance for \mbsgd now is $\frac{\sigma^2}{KS} + (1 - \frac{S}{N})\frac{\zeta^2}{S}$)
    \begin{align}
        \E \|\nabla F(\hat{x}_2)\|^2 \leq  \tilde{\mathcal{O}} (\frac{ \beta (\frac{\beta D^2}{\sqrt{K} R} + \frac{\sigma D}{K^{1/4}} + \zeta D)}{R} + \frac{\beta \sigma D }{\sqrt{S K R}} + \sqrt{1 - \frac{S}{N}}\frac{\beta \zeta D}{\sqrt{SR}})
    \end{align}
    By setting $K \geq \frac{\zeta^4}{\sigma^4}$, $K \geq \frac{\beta^2 D^2}{\zeta R}$,
    \begin{align}
        \E \|\nabla F(\hat{x}_2)\|^2 \leq   \tilde{\mathcal{O}}(\frac{\beta \zeta D}{R} + \frac{\beta \sigma D }{\sqrt{N K R}}+ \sqrt{1 - \frac{S}{N}}\frac{\beta \zeta D}{\sqrt{SR}})
    \end{align}
    Because both \lsgd and \mbsgd do not leave a ball of size $\tilde{\mathcal{O}}(D)$ (seen in \cref{prop:sampled_fedavg} and \cref{prop:convex-sgd}) 
    We see that
    \begin{align}
        \E F(\hat{x}_2) - F(x^*) &\leq \sqrt{\E \|\nabla F(\hat{x}_2)\|^2} \sqrt{\E \|\hat{x}_2 - x^*\|^2} \\
        &\leq \tilde{\mathcal{O}}(\frac{\beta^{1/2} \zeta^{1/2} D^{3/2}}{R^{1/2}} + \frac{\beta^{1/2} \sigma^{1/2} D^{3/2} }{(N K R)^{1/4}} + (1 - \frac{S}{N})^{1/4}\frac{\beta^{1/2} \zeta^{1/2} D^{3/2}}{(SR)^{1/4}})
    \end{align}
\end{proof}
\subsubsection{Sampled \lsgd $\to$ \asg}
\begin{proof}
    By running \lsgd in the setting of \cref{prop:sampled_fedavg} as $\ahead$ and \mbsgd in the setting of \cref{prop:appasgconvex} as $\atail$ we have by setting $K \geq \frac{\zeta^4}{\sigma^4}$, $K \geq \frac{\beta^2 D^2}{\zeta R}$ (because the per-iterate variance for \asg now is $\frac{\sigma^2}{KS} + (1 - \frac{S}{N})\frac{\zeta^2}{S}$),
    \begin{align}
        \E \|\nabla F(\hat{x}_2)\|^2 \leq  \tilde{\mathcal{O}} (\frac{\beta \zeta D}{R^2} + \frac{  \beta D \sigma }{ \sqrt{ S K R}}  + \frac{8 \sigma^2}{ S K R}+ \sqrt{1 - \frac{S}{N}}\frac{\beta \zeta D}{\sqrt{SR}} + (1 - \frac{S}{N}) \frac{\zeta^2}{SR})
    \end{align}
    Because both \lsgd and \asg do not leave a ball of size $\tilde{\mathcal{O}}(D)$ (seen in \cref{prop:sampled_fedavg} and \cref{prop:appasgconvex}) 
    We see that
    \begin{align}
        \E F(\hat{x}_2) - F(x^*) &\leq \sqrt{\E \|\nabla F(\hat{x}_2)\|^2} \sqrt{\E \|\hat{x}_2 - x^*\|^2} \\
        &\leq \tilde{\mathcal{O}}(\frac{\beta^{1/2} \zeta^{1/2} D^{3/2}}{R} + \frac{  \beta^{1/2} D^{3/2} \sigma^{1/2} }{ (S K R)^{1/4}}  + \frac{\sigma D}{ \sqrt{S K R}}+ (1 - \frac{S}{N})^{1/4}\frac{\beta^{1/2} \zeta^{1/2} D^{3/2}}{(SR)^{1/4}} + \sqrt{1 - \frac{S}{N}} \frac{\zeta D}{\sqrt{SR}})
    \end{align}
\end{proof}

\subsubsection{\asg}
\begin{proposition}
    \label{prop:appasgconvex}
    Suppose $F$ is general convex \pcref{asm:convex}, $\beta$-smooth \pcref{asm:smooth}, and each client gradient variance is bounded as $\sigma^2$ \pcref{asm:uniform_variance}.  Then suppose we run \cref{algo:ambsgd} on a modified loss
    \begin{align}
        f_\mu(x;z) = f(x;z) + \frac{\mu}{2} \|x - x^{(0)}\|^2
    \end{align}
    where $x^{(0)}$ is the initial iterate, and 
    \begin{align}
        \mu = \max \{ \frac{2 \beta}{R^2}\log^2(e^2 + R^2) , (\frac{ \beta \sigma^2 }{ 2 \Delta N K R})^{1/2} \}
    \end{align}

    where 
    \begin{align}
        \Phi = \log(\max\{2, \min \{\frac{2 \Delta  \mu NKR }{\sigma^2}, \frac{2 \Delta \mu^2  NKR^3  }{(\beta + \mu) \sigma^2}\})\}
    \end{align}
    with constant stepsize
    \begin{align}
        \eta = \min\{\frac{1}{\beta + \mu}, \frac{\log(\max\{2, \min \{\frac{2 \Delta  \mu NKR }{\sigma^2}, \frac{2 \Delta \mu^2  NKR^3  }{(\beta + \mu) \sigma^2}\})\}}{\mu R^2 }\}.
    \end{align}
    If we return the final iterate
    \begin{align}
        \hat{x} = x^{(R+1)}
    \end{align}
    Then we have the following guarantees:
    \begin{align}
        \E \| \nabla F (\hat{x}) \|^2 &\leq \frac{40 \beta \Delta }{R^2} \log^2 (e^2 + R^2) + 32 (\frac{  \beta^2 D^2 \sigma^2 }{ 2 N K R})^{1/2} \Phi^{3/2}  + \frac{8 \sigma^2}{ N K R} \Phi^{3/2}
    \end{align}
    \begin{align}
        \E \|\hat{x} - x^* \|^2 \leq 18 D^2
    \end{align}
    so long as $R \geq 5$ \footnote{We assume this constant lower bound for technical simplification, as in \citep{yuan2020federatedac}.}

\end{proposition}
\begin{proof}
    Let $F_\mu(x) = F(x) + \frac{\mu}{2} \|x - x^{(0)}\|^2$, where $x^{(0)}$ is the initial iterate.   Also let $x^*_\mu = \argmin_x F_\mu(x)$ and $\Delta_{\mu} := \E [F_\mu(x^{(0)}) - F_\mu(x^*_\mu)]$. 
    
    From \cref{thm:appasg}, we know that running \cref{algo:ambsgd} on $F_\mu$ (noting that $F_\mu$ is $\beta + \mu$-smooth) where $R \geq \sqrt{ \frac{\beta + \mu}{\mu}}$, with constant stepsize
    \begin{align}
        \eta = \min\{\frac{1}{\beta + \mu}, \frac{\log(\max\{e, \min \{\frac{2 \Delta  \mu N K R}{\sigma^2}, \frac{2 \Delta \mu^2  N K R^3  }{(\beta + \mu) \sigma^2}\}\})}{\mu R^2 } \}
    \end{align} 
    we can achieve convergence rate 
    \begin{align}
        \E F_\mu(x^{(R + 1)}) - F_\mu(x^*_\mu)  \leq 2 \Delta_{\mu}  \exp(- \frac{R}{\sqrt{(\beta + \mu)/\mu}}) +  \frac{2 \sigma^2}{\mu N K R} \Phi^{3/2}
    \end{align}
    where 
    \begin{align}
        \Phi = \log(\max\{e, \min \{\frac{2 \Delta  \mu N K R}{\sigma^2}, \frac{2 \Delta \mu^2  N K R^3  }{(\beta + \mu) \sigma^2}\}\})
    \end{align}
    Let $\hat{x} = x^{(R + 1)}$ be the returned iterate.  By \cref{lemma:convsmooth}, 
    \begin{align}
        \E \|\nabla F(\hat{x})\|^2 &\leq 4 \beta (2 \Delta  \exp(- \frac{R}{\sqrt{(\beta + \mu)/\mu}}) +  \frac{2 \sigma^2}{\mu N K R} \Phi^{3/2}) + 8 \mu (\frac{2 \sigma^2}{\mu N K R} \Phi^{3/2} ) + 16 \mu \Delta
    \end{align}
    Combining terms,
    \begin{align}
        \E \|\nabla F(\hat{x})\|^2 &\leq 8\beta  \Delta  \exp(- \frac{R}{\sqrt{(\beta + \mu)/\mu}}) +  \frac{8 \beta \sigma^2}{\mu N K R} \Phi^{3/2}   + \frac{8 \sigma^2}{ N K R} \Phi^{3/2} + 16 \mu \Delta
    \end{align}
    Now make the following settings for $\mu$:
    \begin{align}
        \mu \geq \frac{2 \beta}{R^2}\log^2(e^2 + R^2) \qquad \mu \geq (\frac{ \beta \sigma^2 \Phi^{3/2}}{ 2 \Delta N K R})^{1/2}
    \end{align}
    and $R \geq 5$.  Then from \citep{yuan2020federatedac} Lemma G.5 and Theorem E.1, we have that
    \begin{align}
        \exp(- \frac{R}{\sqrt{(\beta + \mu)/\mu}}) \leq \frac{1}{R^2}
    \end{align}
    So altogether,
    \begin{align}
        \E \| \nabla F (\hat{x}) \|^2 &\leq \frac{40 \beta \Delta }{R^2} \log^2 (e^2 + R^2) + 32 (\frac{  \beta \Delta \sigma^2 \Phi^{3/2}}{ 2 N K R})^{1/2}  + \frac{8 \sigma^2}{ N K R} \Phi^{3/2}
    \end{align}
    To finish the first part of the theorem, observe that with the choice of $\mu \geq \frac{2 \beta}{R^2}\log^2(e^2 + R^2)$, $R \geq \sqrt{\frac{\beta + \mu}{\mu}}$ is always satisfied, and apply $\Delta \leq \beta D^2$ to the second term.

    Now recall again that that
    \begin{align}
        & \E F_\mu(\hat{x}) - F_\mu(x^*_\mu) \\
        &\ \ \ \leq 2 \Delta_{1} \exp(- \frac{R}{\sqrt{(\beta + \mu)/\mu}}) +  \frac{2 \sigma^2}{\mu NKR} \Phi^{3/2}\\
    \end{align}
    By $\beta$-smoothness of $F$ and $\mu$-strong convexity of $F_\mu$,
    \begin{align}
        \E \|\hat{x} - x^*_\mu\|^2 \leq \frac{4 \beta}{\mu} D^2 \exp(- \frac{R}{\sqrt{(\beta + \mu)/\mu}}) +  \frac{4\sigma^2}{\mu^2 NKR} \Phi^{3/2}
    \end{align}
    where $D^2 = \E \|x^{(0)} - x^*\|^2$. By the choice of $\mu$ and $\beta$-smoothness of $F$ (i.e. applying $\Delta_\mu \leq \Delta\leq \beta D^2$ ),
    \begin{align}
        \E \|\hat{x} - x^*_\mu\|^2 \leq 4 D^2
    \end{align}
    Now observe that
    \begin{align}
        F(x_\mu^*) + \|x^{(0)} - x_\mu^*\|^2 \leq F(x^*) + \|x^{(0)} - x^*\|^2
    \end{align}
    which implies that 
    \begin{align}
        \|x^{(0)} - x_\mu^*\|^2 \leq \|x^{(0)} - x^*\|^2
    \end{align}
    And so
    \begin{align}
        \E \|\hat{x} - x^*\|^2 &\leq 3\E \|\hat{x} - x^*_\mu\|^2 + 3 \E \|x^{(0)} - x^*_\mu \|^2 + 3 \E \|x^{(0)} - x^*\|^2 \\
        &\leq 18 D^2
    \end{align}
\end{proof}
\begin{proposition}
    \label{prop:appasgconvex-func}
    Suppose $F$ is general convex \pcref{asm:convex}, $\beta$-smooth \pcref{asm:smooth}, and each client gradient variance is bounded as $\sigma^2$ \pcref{asm:uniform_variance}.  Then suppose we run \cref{algo:ambsgd} on a modified loss
    \begin{align}
        f_\mu(x;z) = f(x;z) + \frac{\mu}{2} \|x - x^{(0)}\|^2
    \end{align}
    where $x^{(0)}$ is the initial iterate, and 
    \begin{align}
        \mu \geq \frac{2 \beta}{R^2}\log^2(e^2 + R^2) \qquad \mu \geq (\frac{ \sigma^2 }{ 2 D^2 N K R})^{1/2}
    \end{align}
    where 
    \begin{align}
        \Phi = \log(\max\{2, \min \{\frac{2 \Delta  \mu NKR }{\sigma^2}, \frac{2 \Delta \mu^2  NKR^3  }{(\beta + \mu) \sigma^2}\})\}
    \end{align}
    with constant stepsize
    \begin{align}
        \eta = \min\{\frac{1}{\beta + \mu}, \frac{\log(\max\{2, \min \{\frac{2 \Delta  \mu NKR }{\sigma^2}, \frac{2 \Delta \mu^2  NKR^3  }{(\beta + \mu) \sigma^2}\})\}}{\mu R^2 }\}.
    \end{align}
    If we return the final iterate
    \begin{align}
        \hat{x} = x^{(R+1)}
    \end{align}
    Then we have the following guarantees:
    \begin{align}
        \E F(\hat{x}) - F(x^*) \leq \min \{ 4 \Delta, \frac{ 3 \beta D^2 }{R^2} \log^2 (e^2 + R^2) \}+ \frac{8 \sigma D}{ \sqrt{N K R}}\Phi^{3/2}
    \end{align}
    \begin{align}
        \E \|\hat{x} - x^*\|^2 \leq 18 D^2 \Phi^{3/2}
    \end{align}
    so long as $R \geq 5$ \footnote{We assume this constant lower bound for technical simplification, as in \citep{yuan2020federatedac}.}

\end{proposition}
\begin{proof}
    Let $F_\mu(x) = F(x) + \frac{\mu}{2} \|x - x^{(0)}\|^2$, where $x^{(0)}$ is the initial iterate.   Also let $x^*_\mu = \argmin_x F_\mu(x)$ and $\Delta_{\mu} := \E [F_\mu(x^{(0)}) - F_\mu(x^*_\mu)]$. 
    
    From \cref{thm:appasg}, we know that running \cref{algo:ambsgd} on $F_\mu$ (noting that $F_\mu$ is $\beta + \mu$-smooth) where $R \geq \sqrt{ \frac{\beta + \mu}{\mu}}$, with constant stepsize
    \begin{align}
        \eta = \min\{\frac{1}{\beta + \mu}, \frac{\log(\max\{e, \min \{\frac{2 \Delta  \mu N K R}{\sigma^2}, \frac{2 \Delta \mu^2  N K R^3  }{(\beta + \mu) \sigma^2}\}\})}{\mu R^2 } \}
    \end{align} 
    we can achieve convergence rate 
    \begin{align}
        \E F_\mu(x^{(R + 1)}) - F_\mu(x^*_\mu)  \leq 2 \Delta_{\mu}  \exp(- \frac{R}{\sqrt{(\beta + \mu)/\mu}}) +  \frac{2 \sigma^2}{\mu N K R} \Phi^{3/2}
    \end{align}
    where 
    \begin{align}
        \Phi = \log(\max\{e, \min \{\frac{2 \Delta  \mu N K R}{\sigma^2}, \frac{2 \Delta \mu^2  N K R^3  }{(\beta + \mu) \sigma^2}\}\})
    \end{align}
    Let $\hat{x} = x^{(R + 1)}$ be the returned iterate.  We have that
    \begin{align}
        \E F_\mu(\hat{x}) - F_\mu(x^*_\mu) \leq 2 \Delta_{\mu}  \exp(- \frac{R}{\sqrt{(\beta + \mu)/\mu}}) +  \frac{2 \sigma^2}{\mu N K R} \Phi^{3/2}
    \end{align}
    From the proof of \cref{lemma:convsmooth} \cref{eq:smooth-func-bound} we have that with the settings for $\mu$,
    \begin{align}
        \E F(\hat{x}) - F(x^*) &\leq 2 \Delta_{\mu}  \exp(- \frac{R}{\sqrt{(\beta + \mu)/\mu}}) +  \frac{2 \sigma^2}{\mu N K R} \Phi^{3/2} + 2 \Delta_\mu + \frac{2 \sigma^2}{\mu N K R}\Phi^{3/2} \\
        &\leq 4 \Delta + \frac{8 \sigma}{ \sqrt{N K R}}\Phi^{3/2}
    \end{align}
    where the last line comes from \cref{lemma:suboptupper}.
    Now observe that 
    \begin{align}
        F_\mu(x_\mu^*) = F(x_\mu^*) + \frac{\mu}{2} \|x_\mu^* - x^{(0)}\|^2 \leq F(x^*) + \frac{\mu}{2} \|x^* - x^{(0)}\|^2
    \end{align}
    So 
    \begin{align}
        F(\hat{x}) - F(x^*) = F_\mu(\hat{x}) - F(x^*) -\frac{\mu}{2}\|\hat{x} - x^{(0)}\|^2 \leq F_\mu(\hat{x}) - F_\mu(x^*_\mu) + \frac{\mu}{2} D^2
    \end{align}
    So we have that 
    \begin{align}
        \E F(\hat{x}) - F(x^*) \leq 2 \beta D^2  \exp(- \frac{R}{\sqrt{(\beta + \mu)/\mu}}) +  \frac{8 \sigma^2}{\mu N K R} \Phi^{3/2} + \frac{\mu}{2} D^2
    \end{align}
    Now recall the following settings for $\mu$:
    \begin{align}
        \mu \geq \frac{2 \beta}{R^2}\log^2(e^2 + R^2) \qquad \mu \geq (\frac{ \sigma^2 }{ 2 D^2 N K R})^{1/2}
    \end{align}
    and $R \geq 5$.  Then from \citep{yuan2020federatedac} Lemma G.5 and Theorem E.1, we have that
    \begin{align}
        \exp(- \frac{R}{\sqrt{(\beta + \mu)/\mu}}) \leq \frac{1}{R^2}
    \end{align}
    So altogether,
    \begin{align}
        \E F(\hat{x}) - F(x^*) \leq \frac{ 3 \beta D^2 }{R^2} \log^2 (e^2 + R^2) + 4 (\frac{  \sigma^2 D^2 \Phi^{3/2}}{ 2  N K R})^{1/2} \Phi^{3/2}
    \end{align}
    To finish the first part of the theorem, observe that with the choice of $\mu \geq \frac{2 \beta}{R^2}\log^2(e^2 + R^2)$, $R \geq \sqrt{\frac{\beta + \mu}{\mu}}$ is always satisfied, and apply $\Delta \leq \beta D^2$ to the second term.

    For the second part of the theorem, simply follow the proof of \cref{prop:appasgconvex}.
\end{proof}
\subsubsection{\lsgd}
\begin{proposition}
    \label{prop:smooth-fedavg}
    Suppose $F$ is general convex \pcref{asm:convex}, $\beta$-smooth \pcref{asm:smooth}, initial function suboptimality is bounded \pcref{asm:subopt}, initial distance to optimum is bounded \pcref{asm:distance}, and each client gradient variance is bounded as $\sigma^2$ \pcref{asm:uniform_variance}.  Then suppose we run \cref{algo:fedavg} on a modified loss
    \begin{align}
        f_\mu(x;z) = f(x;z) + \frac{\mu}{2} \|x - x^{(0)}\|^2
    \end{align}
    where we set $\mu$ to be the smallest number such that
    \begin{align}
        &\mu \geq \frac{16 \beta}{K R}\log(e^2 + K R) \qquad \mu \geq (\frac{\beta \sigma^2}{\Delta N K R})^{1/2} \qquad \mu \geq (\frac{6 \beta^2 \sigma^2}{\Delta K R^2})^{1/3} \qquad \mu \geq (\frac{12 \beta \sigma^2}{\Delta K R^2})^{1/2} \\
        &\mu \geq (\frac{6 \beta^2 \zeta^2}{\Delta R^2})^{1/3} \qquad \mu \geq (\frac{18 \beta \zeta^2}{\Delta R^2})^{1/2}
    \end{align}
    and 
    \begin{align}
        \eta = \min \{\frac{1}{4 (\beta + \mu)}, \frac{\log(\max\{e, \min\{\frac{D^2 N \mu^2 R^2 K^2}{\sigma^2}, \frac{D^2 \mu^2 R^3 K^3}{6 (\beta + \mu) K (\sigma^2 + 2 K \zeta^2)}\})\})}{\mu K R} \}
    \end{align}
    and $\Phi = \log(\max\{e, \min\{\frac{D^2 N \mu^2 R^2 K^2}{\sigma^2}, \frac{D^2 \mu^2 R^3 K^3}{6 (\beta + \mu) K (\sigma^2 + 2 K \zeta^2)}\})$.
    Then we have convergence rate
    \begin{align}
        \E \|\nabla F(\hat{x}) \|^2 &\leq \frac{132 \beta^2 D^2 }{K R} \log(e^2 + K R) + 16 (\frac{\beta^2 \sigma^2 D^2}{N K R})^{1/2} \Phi + 16(\frac{6 \beta^4 \sigma^2 D^4}{K R^2})^{1/3} \Phi^2 + 16 (\frac{12 \beta^2 \sigma^2 D^2}{K R^2})^{1/2} \Phi^2 \\
        & \ \ \ + 16 (\frac{6 \beta^2 \zeta^2 \Delta^2}{ R^2})^{1/3} \Phi^2 + 16 (\frac{18 \beta^2 \zeta^2 D^2}{ R^2})^{1/2} \Phi^2 + \frac{16 \sigma^2}{ N K R} \Phi + \frac{48 \sigma^2}{ K R^2} \Phi^2  + \frac{96 \zeta^2}{ R^2} \Phi^2
    \end{align}
    where $\hat{x}$ is the solution returned from running \cref{algo:fedavg} in the setting of Theorem G.3 in \cite{gorbunov2020local}, so long as $R K \geq 700$ \footnote{This constant lower bound is for technical simplicity, as in \cite{yuan2020federatedac} and can be generalized}.
\end{proposition}
\begin{proof}
    Let $F_\mu(x) = F(x) + \frac{\mu}{2} \|x - x^{(0)}\|^2$, where $x^{(0)}$ is the initial iterate.   Also let $x^*_\mu = \argmin_x F_\mu(x)$ and $\Delta_{\mu} := \E [F_\mu(x^{(0)}) - F_\mu(x^*_\mu)]$.  If we run \cref{algo:fedavg} on $F_\mu$ using constant stepsize (noting that $F_\mu$ is $\beta + \mu$-smooth)
    \begin{align}
        \eta = \min \{\frac{1}{4 (\beta + \mu)}, \frac{\log(\max\{e, \min\{\frac{D^2 N \mu^2 R^2 K^2}{\sigma^2}, \frac{D^2 \mu^2 R^3 K^3}{6 (\beta + \mu) K (\sigma^2 + 2 K \zeta^2)}\})\})}{\mu K R} \}
    \end{align}
    where $\Phi = \log(\max\{e, \min\{\frac{D^2 N \mu^2 R^2 K^2}{\sigma^2}, \frac{D^2 \mu^2 R^3 K^3}{6 (\beta + \mu) K (\sigma^2 + 2 K \zeta^2)}\})$
    then from \cite{gorbunov2020local} Theorem G.3,
    \begin{align}
        \E F_\mu (\hat{x}) - F_\mu(x^*_\mu) \leq 8 (\frac{\beta + \mu}{\mu}) \Delta_\mu \exp(-\frac{KR}{ \frac{8(\beta + \mu)}{\mu}}) + \frac{2 \sigma^2}{\mu N K R} \Phi + \frac{6 (\beta + \mu) \sigma^2}{\mu^2 K R^2} \Phi^2 + \frac{12 (\beta + \mu)\zeta^2}{\mu^2 R^2} \Phi^2
    \end{align}
    By \cref{lemma:convsmooth}, if $RK \geq \frac{8(\beta + \mu)}{\mu} \log(\frac{8(\beta + \mu)}{\mu})$,
    \begin{align}
        \E \|\nabla F(\hat{x}) \|^2 &\leq 4 \beta (\Delta \exp(-\frac{KR}{ \frac{8(\beta + \mu)}{\mu}}) + \frac{2 \sigma^2}{\mu N K R} \Phi + \frac{6 (\beta + \mu) \sigma^2}{\mu^2 K R^2} \Phi^2 + \frac{12 (\beta + \mu)\zeta^2}{\mu^2 R^2} \Phi^2) \\
        & \ \ \ + 8 \mu (\Delta + \frac{2 \sigma^2}{\mu N K R} \Phi + \frac{6 (\beta + \mu) \sigma^2}{\mu^2 K R^2} \Phi^2 + \frac{12 (\beta + \mu)\zeta^2}{\mu^2 R^2} \Phi^2) \\
        &\leq 4 \beta \Delta \exp(-\frac{KR}{ \frac{8(\beta + \mu)}{\mu}}) + \frac{8 \beta\sigma^2}{\mu N K R} \Phi + \frac{48 \beta^2 \sigma^2}{\mu^2 K R^2} \Phi^2 + \frac{96 \beta \sigma^2}{\mu K R^2} \Phi^2 + \frac{48 \beta^2 \zeta^2}{\mu^2 R^2} \Phi^2 + \frac{144 \beta \zeta^2}{\mu R^2} \Phi^2\\
        & \ \ \  + \frac{16 \sigma^2}{ N K R} \Phi + \frac{48 \sigma^2}{ K R^2} \Phi^2  + \frac{96 \zeta^2}{ R^2} \Phi^2 +  8 \mu \Delta \\
    \end{align}
    We now set $\mu$ to be the smallest number such that
    \begin{align}
        &\mu \geq \frac{16 \beta}{K R}\log(e^2 + K R) \qquad \mu \geq (\frac{\beta \sigma^2}{\Delta N K R})^{1/2} \qquad \mu \geq (\frac{6 \beta^2 \sigma^2}{\Delta K R^2})^{1/3} \qquad \mu \geq (\frac{12 \beta \sigma^2}{\Delta K R^2})^{1/2} \\
        &\mu \geq (\frac{6 \beta^2 \zeta^2}{\Delta R^2})^{1/3} \qquad \mu \geq (\frac{18 \beta \zeta^2}{\Delta R^2})^{1/2}
    \end{align}
    Using these settings for $\mu$, and requiring that $R K \geq 700$, 
    \begin{align}
        \E \|\nabla F(\hat{x}) \|^2 &\leq \frac{132 \beta \Delta }{K R} \log(e^2 + K R) + 16 (\frac{\beta \sigma^2 \Delta}{N K R})^{1/2} \Phi + 16(\frac{6 \beta^2 \sigma^2 \Delta^2}{K R^2})^{1/3} \Phi^2 + 16 (\frac{12 \beta \sigma^2 \Delta}{K R^2})^{1/2} \Phi^2 \\
        & \ \ \ + 16 (\frac{6 \beta^2 \zeta^2 \Delta^2}{ R^2})^{1/3} \Phi^2 + 16 (\frac{18 \beta \zeta^2 \Delta}{ R^2})^{1/2} \Phi^2 + \frac{16 \sigma^2}{ N K R} \Phi + \frac{48 \sigma^2}{ K R^2} \Phi^2  + \frac{96 \zeta^2}{ R^2} \Phi^2
    \end{align}
    Using that $\Delta \leq \beta D^2$,
    \begin{align}
        \E \|\nabla F(\hat{x}) \|^2 &\leq \frac{132 \beta^2 D^2 }{K R} \log(e^2 + K R) + 16 (\frac{\beta^2 \sigma^2 D^2}{N K R})^{1/2} \Phi + 16(\frac{6 \beta^4 \sigma^2 D^4}{K R^2})^{1/3} \Phi^2 + 16 (\frac{12 \beta^2 \sigma^2 D^2}{K R^2})^{1/2} \Phi^2 \\
        & \ \ \ + 16 (\frac{6 \beta^2 \zeta^2 \Delta^2}{ R^2})^{1/3} \Phi^2 + 16 (\frac{18 \beta^2 \zeta^2 D^2}{ R^2})^{1/2} \Phi^2 + \frac{16 \sigma^2}{ N K R} \Phi + \frac{48 \sigma^2}{ K R^2} \Phi^2  + \frac{96 \zeta^2}{ R^2} \Phi^2
    \end{align}
    Finally observe that with the condition $\mu \geq \frac{16 \beta}{K R}\log(e^2 + K R)$, $KR \geq \frac{8(\beta + \mu)}{\mu} \log(\frac{8(\beta + \mu)}{\mu})$ is always satisfied.
\end{proof}

\subsection{Chained Algorithms}
\subsubsection{\lsgd $\to$ Smoothed \lsgd}
\begin{theorem}
    \label{thm:convex-lsgd-lsgd}
    Suppose that we run \lsgd \pcref{algo:fedavg} in the setting of \cite{woodworth2020minibatch} Theorem 3, and let its solution be $\hat{x}_1$.  Then we use $\hat{x}_1$ as the initialization to \lsgd, run in the setting of \cref{prop:smooth-fedavg}.  Then we have
    \begin{align}
        &\E \|\nabla F(\hat{x}_2) \|^2 \\
        &\leq \frac{132 \beta^2 D^2 }{K R} \log(e^2 + K R) + 16 (\frac{\beta^2 \sigma^2 D^2}{N K R})^{1/2} \Phi + 16(\frac{6 \beta^4 \sigma^2 D^4}{K R^2})^{1/3} \Phi^2 + 16 (\frac{12 \beta^2 \sigma^2 D^2}{K R^2})^{1/2} \Phi^2 \\
        & \ \ \  + 16 (\frac{18 \beta^2 \zeta^2 D^2}{ R^2})^{1/2} \Phi^2 + \frac{16 \sigma^2}{ N K R} \Phi + \frac{48 \sigma^2}{ K R^2} \Phi^2  + \frac{96 \zeta^2}{ R^2} \Phi^2 \\
        & + 16 (\frac{6 \beta^2 \zeta^2}{ R^2})^{1/3} (\frac{10 \beta D^2}{KR} + \frac{4 \sigma D}{\sqrt{NKR}} + \frac{7 (\beta \sigma^2 D^4)^{1/3}}{K^{1/3} R^{2/3}} + \frac{13 (\beta \zeta^2 D^4)^{1/3}}{R^{2/3}})^{2/3} \Phi^2
    \end{align}
    where $\Phi = \log(\max\{e, \min\{\frac{D^2 N \mu^2 R^2 K^2}{\sigma^2}, \frac{D^2 \mu^2 R^3 K^3}{6 (\beta + \mu) K (\sigma^2 + 2 K \zeta^2)}\})$.
\end{theorem}
\begin{proof}
    If we run \cref{algo:fedavg} in the setting of \cite{woodworth2020minibatch} Theorem 3, with $\hat{x}_{1}$ being the returned solution,
    \begin{align}
        \E F(\hat{x}_{1}) - F(x^*) \leq \frac{10 \beta D^2}{KR} + \frac{4 \sigma D}{\sqrt{NKR}} + \frac{7 (\beta \sigma^2 D^4)^{1/3}}{K^{1/3} R^{2/3}} + \frac{13 (\beta \zeta^2 D^4)^{1/3}}{R^{2/3}}
    \end{align}
    % If we additionally require that 
    % \begin{align}
    %     K \geq \max \{\frac{\beta^{2/3} D^{2/3}}{R^{1/3}}, \frac{\sigma^2 R^{1/3}}{(\beta \zeta^2 )^{2/3} D^{2/3}N }, \frac{\sigma^2}{\zeta^2},  \frac{\sigma^2}{N \beta^2 D^4}, \frac{R^{4/3}\sigma^2}{N (\beta \zeta^2 D^4)^{2/3}}\}
    % \end{align}
    Now if we run \cref{algo:fedavg} in the setting of \cref{prop:smooth-fedavg},
    \begin{align}
        &\E \|\nabla F(\hat{x}_2) \|^2 \\
        &\leq \frac{132 \beta^2 D^2 }{K R} \log(e^2 + K R) + 16 (\frac{\beta^2 \sigma^2 D^2}{N K R})^{1/2} \Phi + 16(\frac{6 \beta^4 \sigma^2 D^4}{K R^2})^{1/3} \Phi^2 + 16 (\frac{12 \beta^2 \sigma^2 D^2}{K R^2})^{1/2} \Phi^2 \\
        & \ \ \ + 16 (\frac{6 \beta^2 \zeta^2}{ R^2})^{1/3} (\E F(\hat{x}_{1}) - F(x^*))^{2/3} \Phi^2 + 16 (\frac{18 \beta^2 \zeta^2 D^2}{ R^2})^{1/2} \Phi^2 + \frac{16 \sigma^2}{ N K R} \Phi + \frac{48 \sigma^2}{ K R^2} \Phi^2  + \frac{96 \zeta^2}{ R^2} \Phi^2
    \end{align}
    where $\Phi = \log(\max\{e, \min\{\frac{D^2 N \mu^2 R^2 K^2}{\sigma^2}, \frac{D^2 \mu^2 R^3 K^3}{6 (\beta + \mu) K (\sigma^2 + 2 K \zeta^2)}\})$.
    \begin{align}
        &\E \|\nabla F(\hat{x}_2) \|^2 \\
        &\leq \frac{132 \beta^2 D^2 }{K R} \log(e^2 + K R) + 16 (\frac{\beta^2 \sigma^2 D^2}{N K R})^{1/2} \Phi + 16(\frac{6 \beta^4 \sigma^2 D^4}{K R^2})^{1/3} \Phi^2 + 16 (\frac{12 \beta^2 \sigma^2 D^2}{K R^2})^{1/2} \Phi^2 \\
        & \ \ \  + 16 (\frac{18 \beta^2 \zeta^2 D^2}{ R^2})^{1/2} \Phi^2 + \frac{16 \sigma^2}{ N K R} \Phi + \frac{48 \sigma^2}{ K R^2} \Phi^2  + \frac{96 \zeta^2}{ R^2} \Phi^2 \\
        & + 16 (\frac{6 \beta^2 \zeta^2}{ R^2})^{1/3} (\frac{10 \beta D^2}{KR} + \frac{4 \sigma D}{\sqrt{NKR}} + \frac{7 (\beta \sigma^2 D^4)^{1/3}}{K^{1/3} R^{2/3}} + \frac{13 (\beta \zeta^2 D^4)^{1/3}}{R^{2/3}} + \frac{4 \sigma }{\sqrt{NK}})^{2/3} \Phi^2
    \end{align}
\end{proof}
\subsubsection{\lsgd $\to$ \mbsgd}
\begin{theorem}
    \label{thm:convex-lsgd-sgd}
    Suppose we run \cref{algo:chaining} where 
    \begin{enumerate}
        \item $\ahead$ is \lsgd \pcref{algo:fedavg} in the setting of \cite{woodworth2020minibatch} Theorem 3 for $R$ rounds
        \item $\atail$ is running \mbsgd \pcref{algo:mbsgd} in the setting of \cref{prop:appsgdconvex-func} with initial distance to optimum estimate of $22D^2$, and then using the result to run \mbsgd \cref{algo:mbsgd} with initial function suboptimality estimate $\Delta_{3/2}$ 
    \end{enumerate}
    where 
    \begin{align}
        \Delta_{3/2} = \min \{\frac{1300 \beta D^2}{KR} + \frac{910 (\beta \sigma^2 D^4)^{1/3}}{K^{1/3} R^{2/3}} + \frac{1690 (\beta \zeta^2 D^4)^{1/3}}{R^{2/3}} + \frac{520 \sigma }{\sqrt{NK}}, \frac{ 792 \beta D^2 }{R} \log (e^2 + R) \} + \frac{580 \sigma D}{ \sqrt{N K R}}
    \end{align}
    We have that 
    \begin{align}
        &\E \|\nabla F(\hat{x}_2)\|^2 \\
        &\leq \min \{\frac{2600 \beta^2 D^2}{KR^2} + \frac{1820 (\beta^4 \sigma^2 D^4)^{1/3}}{K^{1/3} R^{5/3}} + \frac{3380(\beta^4 \zeta^2 D^4)^{1/3}}{R^{5/3}} + \frac{1040 \beta \sigma}{N^{1/2} K^{1/2} R}, \frac{1584 \beta^2 D^2}{R^2} \log(e^2 + R)\} \\
        &+ \frac{594 \beta \sigma D}{N^{1/2} K^{1/2} R^{1/2}}
    \end{align}
    and 
    \begin{align}
        \E \|\hat{x}_2 - x^*\|^2 \leq c D^2
    \end{align}
    where $c$ is some universal constant.
\end{theorem}
\begin{proof}
    If we run $\ahead$ as \cref{algo:fedavg} in the setting of \cite{woodworth2020minibatch} Theorem 3, with $\hat{x}_{1/2}$ being the returned solution,
    \begin{align}
        \E F(\hat{x}_{1/2}) - F(x^*) \leq \frac{10 \beta D^2}{KR} + \frac{4 \sigma D}{\sqrt{NKR}} + \frac{7 (\beta \sigma^2 D^4)^{1/3}}{K^{1/3} R^{2/3}} + \frac{13 (\beta \zeta^2 D^4)^{1/3}}{R^{2/3}}
    \end{align}
    By \cref{lemma:choosefunc},
    \begin{align}
        \E F(\hat{x}_{1}) - F(x^*) \leq \min \{\frac{10 \beta D^2}{KR} + \frac{4 \sigma D}{\sqrt{NKR}} + \frac{7 (\beta \sigma^2 D^4)^{1/3}}{K^{1/3} R^{2/3}} + \frac{13 (\beta \zeta^2 D^4)^{1/3}}{R^{2/3}}, \Delta \} + \frac{4 \sigma }{\sqrt{NK}}
    \end{align}
    Set 
    \begin{align}
        \Delta_1 := \min \{\frac{10 \beta D^2}{KR} + \frac{4 \sigma D}{\sqrt{NKR}} + \frac{7 (\beta \sigma^2 D^4)^{1/3}}{K^{1/3} R^{2/3}} + \frac{13 (\beta \zeta^2 D^4)^{1/3}}{R^{2/3}}, \Delta \} + \frac{4 \sigma }{\sqrt{NK}}
    \end{align}
    Then running $\atail$ as first performing \cref{algo:mbsgd} in the setting of \cref{prop:appsgdconvex-func} for $R$ rounds on $\hat{x}_1$ gives (with output being $\hat{x}_{3/2}$) 
    \begin{align}
        \E F(\hat{x}_{3/2}) - F(x^*) \leq \min \{ 130 \Delta_1, \frac{ 792 \beta D^2 }{R} \log (e^2 + R) \}+ \frac{60 \sigma D}{ \sqrt{N K R}}
    \end{align}
    Where we have that by \cref{fact:fedavg-convex-distance}
    \begin{align}
        \E \|\hat{x}_1 - x^*\|^2 \leq 22 D^2
    \end{align}
    Set 
    \begin{align}
        \Delta_{3/2} = \min \{\frac{1300 \beta D^2}{KR} + \frac{910 (\beta \sigma^2 D^4)^{1/3}}{K^{1/3} R^{2/3}} + \frac{1690 (\beta \zeta^2 D^4)^{1/3}}{R^{2/3}} + \frac{520 \sigma }{\sqrt{NK}}, \frac{ 792 \beta D^2 }{R} \log (e^2 + R) \} + \frac{580 \sigma D}{ \sqrt{N K R}}
    \end{align}
    Now running \mbsgd \pcref{algo:mbsgd} in the setting of \cref{prop:convex-sgd} for $R$ where we let the initial estimate for suboptimality be $\Delta_{3/2}$,
    \begin{align}
        &\E \|\nabla F(\hat{x}_2)\|^2 \\
        &\leq \frac{2 \beta \Delta_{3/2}}{R} + \frac{2 \beta \sigma D }{\sqrt{N K R}} \\
        &\leq \min \{\frac{2600 \beta^2 D^2}{KR^2} + \frac{1820 (\beta^4 \sigma^2 D^4)^{1/3}}{K^{1/3} R^{5/3}} + \frac{3380(\beta^4 \zeta^2 D^4)^{1/3}}{R^{5/3}} + \frac{1040 \beta \sigma}{N^{1/2} K^{1/2} R}, \frac{1584 \beta^2 D^2}{R^2} \log(e^2 + R)\} \\
        &+ \frac{594 \beta \sigma D}{N^{1/2} K^{1/2} R^{1/2}}
    \end{align}
    The guarantee for the distance bound can be obtained by simply observing that each part of the algorithm can only increase the distance to the optimal solution set by a constant.
\end{proof}
\subsubsection{\lsgd $\to$ \asg}
\begin{theorem}
    \label{thm:convex-lsgd-asg}
    Suppose we run \cref{algo:chaining} where 
    \begin{enumerate}
        \item $\ahead$ is \lsgd \pcref{algo:fedavg} in the setting of \cite{woodworth2020minibatch} Theorem 3 for $R$ rounds
        \item $\atail$ starts with running \asg \pcref{algo:ambsgd} for $R$ rounds in the setting of \cref{prop:appasgconvex-func} where the estimate for initial distance to optimum is $22D^2$
        \item $\atail$ finishes with using the result in the previous step to run \asg \pcref{algo:ambsgd} with $R$ rounds in the setting of \cref{prop:appasgconvex} where we let the estimate for function suboptimality be $\Delta_{3/2}$
    \end{enumerate}
    where 
    \begin{align}
        \Delta_{3/2} = \min \{\frac{40 \beta D^2}{KR} + \frac{28 (\beta \sigma^2 D^4)^{1/3}}{K^{1/3} R^{2/3}} + \frac{ 52(\beta \zeta^2 D^4)^{1/3}}{R^{2/3}} + \frac{16 \sigma}{\sqrt{NK}}, \frac{ 66 \beta D^2 }{R^2} \log^2 (e^2 + R^2)\} + \frac{72 \sigma D}{\sqrt{NKR}}
    \end{align}
    We have that 
    \begin{align}
        &\E \|\nabla F(\hat{x}_2)\|^2 \\
        &\leq \min \{\frac{80 \beta^2 D^2}{KR} + \frac{56 (\beta^4 \sigma^2 D^4)^{1/3}}{K^{1/3} R^{8/3}} + \frac{ 104(\beta^4 \zeta^2 D^4)^{1/3}}{R^{8/3}} + \frac{32 \beta \sigma}{\sqrt{NK}}, \frac{ 66 \beta^2 D^2 }{R^4} \log^2 (e^2 + R^2)\} + \frac{144 \beta \sigma D}{\sqrt{NKR}} \Phi^{3/2}
    \end{align}
    and 
    \begin{align}
        \E \|\hat{x}_2 - x^*\|^2 \leq c D^2
    \end{align}
    where $c$ is some universal constant.
\end{theorem}
\begin{proof}
    If we run $\ahead$ as \cref{algo:fedavg} in the setting of \cite{woodworth2020minibatch} Theorem 3, with $\hat{x}_{1/2}$ being the returned solution,
    \begin{align}
        \E F(\hat{x}_{1/2}) - F(x^*) \leq \frac{10 \beta D^2}{KR} + \frac{4 \sigma D}{\sqrt{NKR}} + \frac{7 (\beta \sigma^2 D^4)^{1/3}}{K^{1/3} R^{2/3}} + \frac{13 (\beta \zeta^2 D^4)^{1/3}}{R^{2/3}}
    \end{align}
    By \cref{lemma:choosefunc},
    \begin{align}
        \E F(\hat{x}_{1}) - F(x^*) \leq \min \{\frac{10 \beta D^2}{KR} + \frac{4 \sigma D}{\sqrt{NKR}} + \frac{7 (\beta \sigma^2 D^4)^{1/3}}{K^{1/3} R^{2/3}} + \frac{13 (\beta \zeta^2 D^4)^{1/3}}{R^{2/3}}, \Delta \} + \frac{4 \sigma }{\sqrt{NK}}
    \end{align}
    Set 
    \begin{align}
        \Delta_1 := \min \{\frac{10 \beta D^2}{KR} + \frac{4 \sigma D}{\sqrt{NKR}} + \frac{7 (\beta \sigma^2 D^4)^{1/3}}{K^{1/3} R^{2/3}} + \frac{13 (\beta \zeta^2 D^4)^{1/3}}{R^{2/3}}, \Delta \} + \frac{4 \sigma }{\sqrt{NK}}
    \end{align}
    Then running \asg \pcref{algo:ambsgd} in the setting of \cref{prop:appasgconvex-func} and observing \cref{fact:fedavg-convex-distance} for $R$ rounds where the initial iterate is $\hat{x}_1$ and the output is $\hat{x}_{3/2}$ gives 
    \begin{align}
        \E F(\hat{x}_{3/2}) - F(x^*) \leq \min \{ 4 \Delta_1, \frac{ 66 \beta D^2 }{R^2} \log^2 (e^2 + R^2) \}+ \frac{72 \sigma D}{ \sqrt{N K R}}\Phi^{3/2}
    \end{align}
    where $\Phi = \log(\max\{e, \min \{\frac{2 \Delta  \mu N K R}{\sigma^2}, \frac{2 \Delta \mu^2  N K R^3  }{(\beta + \mu) \sigma^2}\}\})$.
    So altogether,
    \begin{align}
        &\E F(\hat{x}_{3/2}) - F(x^*) \\
        &\leq \min \{\frac{40 \beta D^2}{KR} + \frac{28 (\beta \sigma^2 D^4)^{1/3}}{K^{1/3} R^{2/3}} + \frac{ 52(\beta \zeta^2 D^4)^{1/3}}{R^{2/3}} + \frac{16 \sigma}{\sqrt{NK}}, \frac{ 66 \beta D^2 }{R^2} \log^2 (e^2 + R^2)\} + \frac{72 \sigma D}{\sqrt{NKR}}
    \end{align}
    Set 
    \begin{align}
        \Delta_{3/2} = \min \{\frac{40 \beta D^2}{KR} + \frac{28 (\beta \sigma^2 D^4)^{1/3}}{K^{1/3} R^{2/3}} + \frac{ 52(\beta \zeta^2 D^4)^{1/3}}{R^{2/3}} + \frac{16 \sigma}{\sqrt{NK}}, \frac{ 66 \beta D^2 }{R^2} \log^2 (e^2 + R^2)\} + \frac{72 \sigma D}{\sqrt{NKR}}
    \end{align}
    Now running \asg \pcref{algo:ambsgd} where we let the initial estimate for function suboptimality in \cref{prop:appasgconvex} for $R$ rounds gives
    \begin{align}
        &\E \|\nabla F(\hat{x}_2)\|^2 \\
        &\leq \frac{2 \beta \Delta_{3/2}}{R^2} + \frac{8 \beta \sigma D }{\sqrt{N K R}} \\
        &\leq \min \{\frac{80 \beta^2 D^2}{KR} + \frac{56 (\beta^4 \sigma^2 D^4)^{1/3}}{K^{1/3} R^{8/3}} + \frac{ 104(\beta^4 \zeta^2 D^4)^{1/3}}{R^{8/3}} + \frac{32 \beta \sigma}{\sqrt{NK}}, \frac{ 66 \beta^2 D^2 }{R^4} \log^2 (e^2 + R^2)\} + \frac{144 \beta \sigma D}{\sqrt{NKR}} \Phi^{3/2} \\
        &+ \frac{8\sigma^2}{\mu K R}
    \end{align}
    The guarantee for the distance bound can be obtained by simply observing that each part of the algorithm can only increase the distance to the optimal solution set by a constant.
\end{proof}

\begin{fact}
    \label{fact:fedavg-convex-distance}
    Suppose $F_i$'s are general convex \pcref{asm:convex} and $\beta$-smooth \pcref{asm:smooth}.  If we run \cref{algo:fedavg} with constant stepsize 
    \begin{align}
        \eta = \min \{\frac{1}{10 \beta}, \frac{D \sqrt{N}}{\sigma \sqrt{KR}}, (\frac{D^2}{\beta K^2 R \sigma^2})^{1/3}, (\frac{D^2}{\beta K^3 R \zeta^2})^{1/3} \}
    \end{align}
    and return 
    \begin{align}
        \hat{x} = \frac{1}{NKR} \sum_{i=1}^N \sum_{k=1}^K \sum_{r=0}^{R-1} x_{i,k}^{(r)}
    \end{align}
    as the solution, then we have the following two guarantees:
    \begin{align}
        \E[F(\hat{x}) - F(x^*)] \leq \frac{10 \beta D^2}{KR} + \frac{4 \sigma D}{\sqrt{NKR}} + \frac{7 (\beta \sigma^2 D^4)^{1/3}}{K^{1/3} R^{2/3}} + \frac{13 (\beta \zeta^2 D^4)^{1/3}}{R^{2/3}}
    \end{align}
    \begin{align}
        \E \|\hat{x} - x^*\|^2 \leq 22 D^2
    \end{align}
\end{fact}
\begin{proof}
    From \cite{woodworth2020minibatch} Theorem 3, running FedAvg (\cref{algo:fedavg}) with constant stepsize 
    \begin{align}
        \eta = \min \{\frac{1}{10 \beta}, \frac{D \sqrt{N}}{\sigma \sqrt{KR}}, (\frac{D^2}{\beta K^2 R \sigma^2})^{1/3}, (\frac{D^2}{\beta K^3 R \zeta^2})^{1/3} \}
    \end{align}
    and letting the output returned by the algorithm be 
    \begin{align}
        \hat{x} = \frac{1}{NKR} \sum_{i=1}^N \sum_{k=1}^K \sum_{r=0}^{R-1} x_{i,k}^{(r)}
    \end{align}
    we have the following guarantee:
    \begin{align}
        \E[F(\hat{x}) - F(x^*)] \leq \frac{10 \beta D^2}{KR} + \frac{4 \sigma D}{\sqrt{NKR}} + \frac{7 (\beta \sigma^2 D^4)^{1/3}}{K^{1/3} R^{2/3}} + \frac{13 (\beta \zeta^2 D^4)^{1/3}}{R^{2/3}}
    \end{align}
    Define $\bar{x}_{Kr + k} = \frac{1}{N} \sum_{i=1}^N x_{i,k}^{(r)}$.  Then we know from \cite{woodworth2020minibatch} Eq. 128 that
    \begin{align}
        \E[F(\bar{x}_{t}) - F(x^*)] \leq \frac{\E \|\bar{x}_{t} - x^*\|^2 - \E\|\bar{x}_{t+1} - x^*\|^2}{\eta} + \frac{3 \sigma^2 \eta}{N} + 6 \beta K \sigma^2 \eta^2 + 12 \beta K^2 \eta^2 \zeta^2
    \end{align}
    Therefore, we have by convexity of $F$ that for any $T$:
    \begin{align}
        &\E[F(\frac{1}{T} \sum_{t=0}^{T-1} \bar{x}_t) - F(x^*)] \\
        & \ \ \ \leq \frac{1}{\eta T} (\E \|x^{(0)} - x^*\|^2 - \E\|\bar{x}_{T} - x^*\|^2) + \frac{3 \sigma^2 \eta}{N} + 6 \beta K \sigma^2 \eta^2 + 12 \beta K^2 \eta^2 \zeta^2
    \end{align}
    Rearranging, we get (along with the fact that $F(\frac{1}{T} \sum_{t=0}^{T-1} \bar{x}_t) - F(x^*) \geq 0$ and that $T \leq KR$)
    \begin{align}
        \E\|\bar{x}_{T} - x^*\|^2 \leq D^2 + \frac{3\sigma^2 \eta^2 K R}{N} + 6 \beta K^2 R \sigma^2 \eta^3  + 12 \beta K^3 R \eta^3  \zeta^2
    \end{align}
    Recalling the stepsize choice
    \begin{align}
        \eta = \min \{\frac{1}{10 \beta}, \frac{D \sqrt{N}}{\sigma \sqrt{KR}}, (\frac{D^2}{\beta K^2 R \sigma^2})^{1/3}, (\frac{D^2}{\beta K^3 R \zeta^2})^{1/3} \}
    \end{align}
    We obtain
    \begin{align}
        \E \|\bar{x}_{T} - x^*\|^2 \leq 22 D^2
    \end{align}
    for any $T$.  Because $\hat{x} = \frac{1}{KR} \sum_{T = 0}^{KR - 1} \bar{x}_T$, we also have by Jensen's inequality
    \begin{align}
        \E \|\hat{x} - x^*\|^2 \leq \frac{1}{KR} \sum_{T = 0}^{KR - 1} \E \|\bar{x}_{T} - x^*\|^2 \leq 22 D^2
    \end{align}
\end{proof}
