# Supplementary material for: FedChain: Chained Algorithms for Near-Optimal Communication Cost in Federated Learning
Source: arXiv:2108.06869 source file (2023-04-16)
Supplement: Supplementary file 2 [file partial.tex]

%!TEX root = ./main.tex
\section{Discussion on Partial Client Participation}
\label{sec:partial}
\begin{algorithm}[H]
	\caption{(Simplified) Partial Participation FedAvg$\to$SGD}
	\label{algo:partialfedavgsgd}
	\begin{algorithmic}
		\STATE \textbf{Input:} Number of local steps $K$, rounds $R$, stepsize $\eta^{(1)}$, stepsize sequence $\{\eta^{(2)}_r\}_{1 \leq r \leq R - 1}$, initial point ${x}^{(0)}$, maximum number of clients to sample per round $S$
        \STATE Server chooses a client $j \in [N]$ uniformly randomly
        \STATE Server \textbf{communicates} $x^{(0)}$ to client $j$
        \STATE Client $j$ sets $x_{j,0}^{(0)} = 0$
        \FOR{$k = 0, \dots, K-1$}
            \STATE $x_{j,k + 1}^{(0)} \gets x_{j,k}^{(0)} - \eta^{(1)} \cdot \nabla F_i(x_{j,k}^{(0)})$
        \ENDFOR
        \STATE Client $j$ sets $\bar{x}_{j,K} = \frac{1}{W_K} \sum_{k=1}^{K} w_k x_{j,k}^{(0)}$ where $w_k = (1 - \frac{\eta^{(1)} \mu}{4})^{-k}$ and $W_K = \sum_{k=1}^K w_k$
        \STATE Client $j$ \textbf{communicates} $\bar{x}_{j,K}$ to server
        \STATE Server sets $x^{(1)} \gets \bar{x}_{j,K}$
        \FOR{$r = 1, \dots, R-1$}
            \STATE Sample clients $\mathcal{S} \subseteq [N]$ of size $S$
            \STATE $x^{(r + 1)} \gets x^{(r)} - \eta^{(2)}_r \cdot \frac{1}{SK} \sum_{i \in \mathcal{S}, 1 \leq k \leq K}\nabla F_i(x^{(r)})$
        \ENDFOR
	\end{algorithmic}
\end{algorithm}

In this section we discuss the rates our framework can achieve if only a subsample of clients is selected.  For simplicity's sake, we will assume that $\sigma^2 = 0$, e.g. there is no stochasticity in the client gradient computations.  The algorithm we will study is as follows.

\begin{enumerate}
    \item We run SGD on one client for K local steps in the first round.
    \item We take the solution from the end of step (1) and run SGD from the server.  Precisely, each round we use the average of $K$ gradients taken from each of the $S$ uniformly sampled clients as the unbiased gradient for SGD.
\end{enumerate}

We write out the algorithm explicitly in \cref{algo:partialfedavgsgd}.  

We choose to run the FedAvg component of the algorithm with one client sampled and for only one round because analyzing this simple case already conveys the nature of the gain we receive from our framework in the partial participation setting.

We start by analyzing an upper bound on suboptimality after step (1).  For our proof, we need the following definitions: 
\begin{align}
    \hat{\zeta}^2 := \sup_{i,x} \|\nabla F(x) - \nabla F_i(x) \|^2,
    \qquad
    \hat{\zeta}^2_* := \sup_i \|\nabla F_i(x^*) \|^2,
    \label{def:maxheterogeneity}
\end{align}

\begin{theorem}
    \label{thm:partial}
    Let $\bar{x}_{j,K} = \frac{1}{W_K} \sum_{k=1}^{K} w_k x_{j,k}^{(0)}$ where $w_k = (1 - \frac{\eta^{(1)} \mu}{4})^{-k}$ and $W_K = \sum_{k=1}^K w_k$, where $x_{j,k}^{(0)}$ are generated in the following way:
    \begin{align}
        x_{j,k}^{(0)} \gets x_{j,k-1}^{(0)} - \eta_1 \cdot \nabla F_j(x_{j,k-1}^{(0)})
    \end{align}
    where $x_{j,0}^{(0)} = x^{(0)}$.
    For any $j \in [N]$, $\bar{x}_{j,K}$ satisfies
    \begin{align}
        F(\bar{x}_{j,K}^{(0)}) - F(x^*) \leq \frac{4 \beta^2}{\mu} \|x^{(0)} - x^*\|^2 \exp(-\frac{K}{4 \kappa^2}) + \frac{2 \hat{\zeta}^2}{\mu}
    \end{align}
    as long as $\eta^{(1)} \leq \frac{\mu}{8 \beta^2}$.
\end{theorem}
\begin{proof}
    Shorthand $x_{j,k}^{(0)}$ as $x_k$ and $\eta^{(1)}$ as $\eta_1$ for the duration of this proof.  Then
    \begin{align}
        \label{eq:partialgd}
        \|x_k - x^*\|^2 &= \|x_{k-1} - \eta_1 \nabla F_j(x_k) - x^*\|^2 \\
        &= \|x_{k-1} - x^*\|^2 - 2 \eta_1 \langle \nabla F_j(x_k), x_k - x^* \rangle + \eta_1^2 \|\nabla F_j(x_k)\|^2 
    \end{align}
    We start by bounding the middle term of \cref{eq:partialgd}.
    \begin{align}
        \label{eq:middleterm}
        - 2 \eta_1 \langle \nabla F_j(x_k), x_k - x^* \rangle  &= -2 \eta_1(\langle \nabla  F(x_k), x_k - x^* \rangle + \langle \nabla  F_j(x_k) - F(x_k), x_k - x^* \rangle)
    \end{align}
    The first term of \cref{eq:middleterm} can be upper bounded using strong convexity \cref{asm:strongconvex}:
    \begin{align}
        -\langle \nabla  F(x_k), x_k - x^* \rangle \leq -(F(x_k) - F(x^*) + \frac{\mu}{2}\|x_k - x^*\|^2)
    \end{align}
    The second term can be upper bounded using the Fenchel-Young inequality:
    \begin{align}
        -\langle \nabla  F_j(x_k) - F(x_k), x_k - x^* \rangle &\leq \frac{1}{ \mu} \|F_j(x_k) - F(x_k)\|^2 + \frac{\mu}{4} \|x_k - x^*\|^2 \\
        &\leq \frac{\hat{\zeta}^2}{ \mu}  + \frac{\mu}{4} \|x_k - x^*\|^2
    \end{align}
    Where in the last inequality we used the definition of $\hat{\zeta}^2$.

    Next, we upper bound the third term of \cref{eq:partialgd}.
    \begin{align}
        \eta_1^2\|\nabla F_j(x_k)\|^2 &= 2 \eta_1^2\|\nabla F_j(x_k) - F_j(x^*)\|^2 + 2\eta_1^2\|\nabla F_j(x^*)\|^2 \\
        &\leq 2 \eta_1^2 \beta^2 \|x_k - x^*\|^2 + 2 \eta_1^2 \hat{\zeta}_*^2
    \end{align}
    where in the last step we used smoothness \cref{asm:smooth} for the first term and the definition of $\hat{\zeta}_*^2$ for the second term.

    We can substitute all our upper bounds into \cref{eq:partialgd} to get

    \begin{align}
        & \|x_k - x^*\|^2 \\
        &\leq (1 - \eta_1 \mu + \frac{\eta_1 \mu}{2} + 2 \eta_1^2 \beta^2)\|x_{k-1} - x^*\|^2 - 2\eta_1(F(x_k) - F(x^*)) + \frac{2 \eta_1 \hat{\zeta}^2}{\mu} + 2 \eta_1^2 \hat{\zeta}_*^2
    \end{align}
    Setting $\eta_1 \leq \frac{\mu}{8\beta^2}$, we know that $2 \eta_1^2 \beta^2 \leq \frac{\eta_1 \mu}{4}$ and that $2 \eta_1^2 \hat{\zeta}_*^2 \leq \frac{ \eta_1 \mu \hat{\zeta}_*^2}{4 \beta^2} \leq \frac{ \eta_1 \hat{\zeta}_*^2}{4 \mu} \leq \frac{ \eta_1 \hat{\zeta}^2}{4 \mu}$.  So we have 
    \begin{align}
        & \|x_k - x^*\|^2 \\
        &\leq (1 - \frac{\eta_1 \mu}{4})\|x_{k-1} - x^*\|^2 - 2\eta_1(F(x_k) - F(x^*)) + \frac{3 \eta_1 \hat{\zeta}^2}{\mu} 
    \end{align}
    And rearranging, 
    \begin{align}
        F(x_k) - F(x^*) \leq \frac{(1 - \frac{\eta_1 \mu}{4})\|x_{k-1} - x^*\|^2 - \|x_k - x^*\|^2}{2 \eta_1} + \frac{2 \hat{\zeta}^2}{\mu}
    \end{align}
    Using convexity of $F$, and letting $\bar{x}_K := \bar{x}_{j,K}$, we know if $w_k = (1 - \frac{\eta_1 \mu}{4})^{-k}$, then
    \begin{align}
        F(\bar{x}_{K}) - F(x^*) &\leq \frac{1}{W_K} \sum_{k=1}^{K} w_k (F(x_k) - F(x^*)) \\
        &\leq \frac{1}{2 \eta_1 W_K} \sum_{k=1}^{K} w_k [(1 - \frac{\eta_1 \mu}{4})\|x_{k-1} - x^*\|^2 - \|x_k - x^*\|^2] + \frac{2 \hat{\zeta}^2}{\mu} \\
        &\leq \frac{1}{2 \eta_1 W_K} (\|x_0 - x^*\|^2) + \frac{2 \hat{\zeta}^2}{\mu}
    \end{align}
    Noting again that $\eta_1 \leq \frac{\mu}{8 \beta^2}$ and that $\frac{1}{W_K} \leq \frac{1}{w_K} \leq (1 - \frac{\eta_1\mu}{4})^K$, we have 
    \begin{align}
        F(\bar{x}_{K}) - F(x^*) &\leq \frac{4 \beta^2}{\mu} \|x_0 - x^*\|^2 (1 - \frac{\eta_1 \mu}{4})^K + \frac{2 \hat{\zeta}^2}{\mu} \\
        &\leq \frac{4 \beta^2}{\mu} \|x_0 - x^*\|^2 \exp(-\frac{K}{4 \kappa^2}) + \frac{2 \hat{\zeta}^2}{\mu}
    \end{align}
\end{proof}
\begin{remark}
    Surprisingly, \cref{thm:partial} is the only known rate (to our knowledge) for FedAvg (even running for one round, only sampling one client, and assuming noiseless gradients) under partial participation in the heterogeneous client setting that is tight in the following sense: given large enough $K$, only one communication round is needed to get convergence to the global solution if $\zeta^2 = 0$ (which implies $\hat{\zeta}^2 = 0$, e.g. completely homogeneous clients).  Other rates for FedAvg in partial participation, such as those in \citep{karimireddy2020scaffold,stich2019error} do not have this property.  The work on federated optimization in the partial participation setting is fairly immature, and is an important future direction.
\end{remark}

\begin{remark}
    One might expect the $\frac{\hat{\zeta}^2}{\mu}$ term to shrink with $S$, e.g. be something like $\frac{\hat{\zeta}^2}{\mu S}$, as this is true for partial-participation SGD \cite{woodworth2020minibatch}.  However, the evidence points towards this not being true for partial participation FedAvg, because in the rate for full participation FedAvg, the heterogeneity term does not shrink with $N$.
\end{remark}

Using this, we get a convergence rate for FedAvg$\to$SGD (\cref{algo:partialfedavgsgd}) in the partial participation setting:
\begin{theorem}
    Let $x^{(1)} = \bar{x}_{j,K}$, as specified from \cref{thm:partial}.  Let the total round budget be $R + 1$.  Then if we have the following (i.e. running partial participation SGD with $x^{(1)}$ as the initial point) \citep{woodworth2020minibatch})
    \begin{enumerate}
        \item If $R > \frac{4 \beta}{\mu}$ and $r - 1 < \lceil \frac{R}{2} \rceil$: 
        $\eta^{(2)}_{r} = \eta_g =  \frac{1}{4 \beta}$, 
        $w_{r} = 0$ 
        \item  If $R > \frac{4 \beta}{\mu}$ and $r - 1\geq \lceil R/2 \rceil$: $\eta^{(2)}_{r} = \frac{2}{\mu(\kappa - R - \lceil \frac{R}{2} \rceil)}$, $w_{r} = (\kappa + r - \lceil \frac{R}{2} \rceil)^2$	
        \item If $R \leq \frac{4 \beta}{\mu}$:
        $\eta^{(2)}_{r} = \frac{1}{4\beta}$, 
        $w_{r} = (1 - \mu \eta_g)^{-(r + 1)}$.
    \end{enumerate}
    Where \cref{algo:partialfedavgsgd} returns 
    \begin{align}
        \hat{x} = \sum_{r = 2}^{R+1} w_r x^{(r)} 
    \end{align}
    Then we have the following convegence rate for \cref{algo:partialfedavgsgd} if $K \geq \kappa^2 \log \frac{\beta^2 D^2}{\hat{\zeta}^2}$:
    \begin{align}
        \E[F(\hat{x}) - F(x^*)] \leq O( \frac{\hat{\zeta}^2}{\mu} \exp(-\frac{R}{\sqrt{\kappa}}) + (1 - \frac{S}{N}) \frac{\zeta^2}{\mu S R})
    \end{align}
\end{theorem}
\begin{proof}
The rate for running partial participation SGD with $x^{(1)}$ as the initial point which samples $S$ clients per round from \citep{woodworth2020minibatch} (eq. 18) is

\begin{align}
    \label{eq:partialsgd}
    \E[F(x^{(r)}) - F(x^*)] \leq O(\kappa [\E F(x^{(1)}) - F(x^*)]\exp(-\frac{R}{\kappa}) + (1 - \frac{S}{N}) \frac{\zeta_*^2}{\mu S R})
\end{align}
We can substitute for $\E F(x^{(1)}) - F(x^*)$ the final suboptimality from \cref{thm:partial}, which gives 
\begin{align*}
    \E[F(x^{(r)}) - F(x^*)] \leq O(\kappa (\frac{\beta^2}{\mu} \|x^{(0)} - x^*\|^2 \exp(-\frac{K}{\kappa^2}) + \frac{\hat{\zeta}^2}{\mu}) \exp(-\frac{R}{\kappa}) + (1 - \frac{S}{N}) \frac{\zeta_*^2}{\mu S R})
\end{align*}

If we set $K \geq \kappa^2 \log \frac{\beta^2 D^2}{\hat{\zeta}^2}$ where $D^2 \leq \|x^{(0)} - x^*\|^2$, then the convergence rate becomes 

\begin{align}
    \label{eq:partialfinalminibatch}
    \E[F(x^{(r)}) - F(x^*)] \leq O( \frac{\kappa \hat{\zeta}^2}{\mu} \exp(-\frac{R}{\kappa}) + (1 - \frac{S}{N}) \frac{\zeta_*^2}{\mu S R})
\end{align}
\end{proof}
It is easy to check that if we had used Nesterov acceleration in the second phase (like in \citep{woodworth2020minibatch}), the rate would instead be 
\begin{align}
    \label{eq:partialfinal}
    \E[F(x^{(r)}) - F(x^*)] \leq O( \frac{\hat{\zeta}^2}{\mu} \exp(-\frac{R}{\sqrt{\kappa}}) + (1 - \frac{S}{N}) \frac{\zeta^2}{\mu S R})
\end{align}

For both partial SGD and partial FedAvg $\to$ SGD (\cref{eq:partialsgd} vs \cref{eq:partialfinalminibatch}), we see that the rate in \cref{eq:partialfinal} is better if $\frac{\hat{\zeta}}{\mu} \leq \Delta$.  Similar is true with acceleration.

On the other hand, our new rates \cref{eq:partialfinalminibatch} and \cref{eq:partialfinal} improves on the rate for FedAvg \cref{thm:partial} because our errors shrink with $S$ and with $R$, supposing all the measures of heterogeneity $\zeta, \hat{\zeta}, \zeta_*, \hat{\zeta}_*$ are of the same order.  However, the magnitude of improvement is not as substantial as in the full participation case: here we only improve by a factor of $R$, while in the full participation case we improved exponentially.

It is unclear if our algorithm/analysis is suboptimal here, because there is no known lower bound for partial participation FL in the heterogeneous setting (unlike for full participation).  Understanding the limits of optimization in FL when clients are sampled and client data is heterogeneous is important future work.
