# Supplementary material for: FedChain: Chained Algorithms for Near-Optimal Communication Cost in Federated Learning
Source: arXiv:2108.06869 source file (2023-04-16)
Supplement: Supplementary file 3 [file plproofs.tex]

%!TEX root = ./main.tex
\section{Proofs under the PL condition}
\subsection{\mbsgd}
\begin{proposition}
    \label{thm:plsgd}
    Given $\mu$-PL \pcref{asm:pl}, $\beta$-smoothness \pcref{asm:smooth} of $F$, and uniform client gradient variance bound \pcref{asm:uniform_variance}, upper bound on initial function suboptimality \pcref{asm:subopt}, then \mbsgd \pcref{algo:mbsgd} with
    \begin{align}
        \eta = \min \{ \frac{1}{\beta}, \frac{\log(\max\{e, \frac{2 \mu^2 \Delta NKR}{\beta \sigma^2}\})}{\mu R} \}
    \end{align}
    and defining
    \begin{align}
        \Phi := \log(\max\{e, \frac{2 \mu^2 \Delta NKR}{\beta \sigma^2}\})
    \end{align}
    Achieves convergence rate
    \begin{align}
        \E F(x^{(R)}) - F(x^*) \leq \Delta \exp(-\frac{R}{\kappa}) + \frac{\beta \sigma^2}{\mu^2 N K R} \Phi
    \end{align}
\end{proposition}
\begin{proof}
    Using $\beta$-smoothness of $F$ \pcref{asm:smooth}, we have
    \begin{align}
        F(x^{(r + 1)}) - F(x^{(r)}) \leq \langle \nabla F(x^{(r)}), x^{(r + 1)} - x^{(r)} \rangle + \frac{\beta}{2} \|x^{(r + 1)} - x^{(r)}\|^2
    \end{align}
    Using the update rule $x^{(r+1)} = x^{(r)} - \eta g^{(r)}$, where $ g^{(r)}$ is defined as
    \begin{align}
        g^{(r)} := \frac{1}{NK} \sum_{i=1}^N \sum_{k=1}^K g_{i,k}^{(r)}
    \end{align}
    we have that 
    \begin{align}
        F(x^{(r + 1)}) - F(x^{(r)}) \leq -\eta \langle \nabla F(x^{(r)}), g^{(r)} \rangle + \frac{\beta \eta^2}{2} \|g^{(r)}\|^2
    \end{align}
    Taking expectations of both sides conditioned on the $r$-th step,
    \begin{align}
        \E_r F(x^{(r + 1)}) - F(x^{(r)}) \leq -\eta \|F(x^{(r)})\|^2 + \frac{\beta \eta^2}{2} \E_r \|g^{(r)}\|^2
    \end{align}
    Observe that 
    \begin{align}
        \E_r \|g^{(r)}\|^2 = \E_r \|g^{(r)} - \nabla F(x^{(r)}) \|^2 + \E_r \| \nabla F(\x{r})\|^2
    \end{align}
    Which gives
    \begin{align}
        \E_r F(x^{(r + 1)}) - F(x^{(r)}) \leq -\eta(1 - \frac{\beta \eta}{2}) \|F(x^{(r)})\|^2 + \frac{\beta \eta^2}{2} \E_r \|g^{(r)} - \nabla F(x^{(r)}) \|^2
    \end{align}
    Letting $\eta \leq \frac{1}{\beta}$,
    \begin{align}
        \E_r F(x^{(r + 1)}) - F(x^{(r)}) \leq -\frac{\eta}{2} \|F(x^{(r)})\|^2 + \frac{\beta \eta^2}{2} \E_r \|g^{(r)} - \nabla F(x^{(r)}) \|^2
    \end{align}
    From \cref{lemma:minibatchvariance} using \pcref{asm:uniform_variance}, we can get
    \begin{align}
        \E_r F(x^{(r + 1)}) - F(x^{(r)}) \leq -\frac{\eta}{2} \|F(x^{(r)})\|^2 + \frac{\beta \sigma^2 \eta^2 }{2 NK} 
    \end{align}
    By $\mu$-PL \pcref{asm:pl}, we have that
    \begin{align}
        \E_r F(x^{(r + 1)}) - F(x^{(r)}) \leq -\eta \mu(F(x^{(r)}) - F(x^*)) + \frac{\beta \sigma^2 \eta^2 }{2 NK} 
    \end{align}
    Rearranging,
    \begin{align}
        \E_r F(x^{(r + 1)}) - F(x^*) \leq (1 - \eta \mu)(F(x^{(r)}) - F(x^*)) + \frac{\beta \sigma^2 \eta^2 }{2 NK} 
    \end{align}
    Subtracting $\frac{\beta \sigma^2 \eta}{2 \mu}$ from both sides,
    \begin{align}
        \E_r F(x^{(r + 1)}) - F(x^*) - \frac{\beta \sigma^2 \eta}{2 \mu NK}\leq (1 - \eta \mu)(F(x^{(r)}) - F(x^*) - \frac{\beta \sigma^2 \eta}{2 \mu NK})
    \end{align}
    Which, upon unrolling the recursion, gives us
    \begin{align}
        \E F(x^{(R)}) - F(x^*)  \leq \Delta \exp(-\eta \mu R) + \frac{\beta \sigma^2 \eta }{2 \mu NK} 
    \end{align}
    Now, if we choose stepsize 
    \begin{align}
        \eta = \min \{ \frac{1}{\beta}, \frac{\log(\max\{e, \frac{2 \mu^2 \Delta NKR}{\beta \sigma^2}\})}{\mu R} \}
    \end{align}
    Letting 
    \begin{align}
        \Phi = \log(\max\{e, \frac{2 \mu^2 \Delta NKR}{\beta \sigma^2}\})
    \end{align}
    Then the final convergence rate is 
    \begin{align}
        \E F(x^{(R)}) - F(x^*) \leq \Delta \exp(-\frac{R}{\kappa}) + \frac{\beta \sigma^2}{\mu^2 N K R} \Phi
    \end{align}
\end{proof}
\subsection{M-\mbsgd}
\begin{proposition}
    \label{thm:pl-m-sgd}
    Suppose we run M-\mbsgd \pcref{algo:m-mbsgd}.  Then given $\mu$-PL \pcref{asm:pl} of $F$ (or $\mu$-strong convexity \pcref{asm:strongconvex}), $\beta$-smoothness of $F_i$'s \pcref{asm:smooth}, upper bound on initial function suboptimality \pcref{asm:subopt}, and a uniform upper bound of variance $\sigma^2$ \pcref{asm:uniform_variance}, if we choose $\eta_s = \frac{\eta}{2^s}$ and $R_s = \frac{2^s \log(4)}{\mu \eta}$

    with 

    \begin{align}
        \eta = \min \{ \frac{1}{\beta}, \frac{\log(\max\{e, \frac{2 \mu^2 \Delta NKR}{\beta \sigma^2}\})}{\mu R} \}
    \end{align}
    and letting
    \begin{align}
        \Phi = \log(\max\{e, \frac{2 \mu^2 \Delta NKR}{\beta \sigma^2}\})
    \end{align}

    Then we have 
    \begin{align}
        \E F(x^{(s, R_s)}) - F(x^*) \leq \frac{1}{2^{s-1}}(\Delta \exp(-\frac{R_1}{\kappa}) + \frac{\beta \sigma^2}{ \mu^2 N K R} \Phi)
    \end{align}
    also, if $R \geq \kappa$ and $s$ is constant, then
    \begin{align}
        \E F(x^{(s, R_s)}) - F(x^*) \leq c (\Delta \exp(-\frac{R}{C \kappa}) + \frac{\beta \sigma^2 }{\mu^2 N K R} \Phi)
    \end{align}
    for some universal constants $c,C$.
\end{proposition}
\begin{proof}
    Recall that from the proof of \pcref{thm:plsgd},
    \begin{align}
        \E F(x^{(1, R_1)}) - F(x^*)  \leq \Delta \exp(-\eta \mu R_1) + \frac{\beta \sigma^2 \eta_1 }{2 \mu NK} 
    \end{align}
    Now recalling the definition of $\eta_s = \frac{\eta}{2^s}$ and $R_s = \frac{2^s \log(4)}{\mu \eta}$, and letting 
    \begin{align}
        \text{err}_s = \E F(x^{(s, R_s)}) - F(x^*)
    \end{align}
    we want to prove by induction that 
    \begin{align}
        \text{err}_s \leq \frac{1}{2^{s-1}}(\Delta \exp(-\eta \mu R_1) + \frac{\beta \sigma^2 \eta_1 }{2 \mu NK})
    \end{align}
    The base case is already proven for $s=1$, so we move on to the inductive case.
    \begin{align}
        \text{err}_{s+1} &\leq \frac{1}{4}(\frac{1}{2^{s-1}}(\Delta \exp(-\eta \mu R_1) + \frac{\beta \sigma^2 \eta_1 }{2 \mu NK})) + \frac{\beta \sigma^2 \eta}{2 \mu N K 2^{s+1}} \\
        &\leq (\frac{1}{2^{s+1}}(\Delta \exp(-\eta \mu R_1) + \frac{\beta \sigma^2 \eta_1 }{2 \mu NK 2^{s+1}})) + \frac{\beta \sigma^2 \eta}{2 \mu N K 2^{s+1}} \\
        &\leq \frac{1}{2^{s}}(\Delta \exp(-\eta \mu R_1) + \frac{\beta \sigma^2 \eta_1 }{2 \mu NK})
    \end{align}
    which completes the induction.  If $s$ is a constant and $K \geq \kappa$, then for universal constants $c, C$ we have that 
    \begin{align}
        \text{err}_s \leq c (\Delta \exp(-\eta \mu (R/C)) + \frac{\beta \sigma^2 \eta}{2 \mu N K})
    \end{align}
    Now, if we choose stepsize 
    \begin{align}
        \eta = \min \{ \frac{1}{\beta}, \frac{\log(\max\{e, \frac{2 \mu^2 \Delta NKR}{\beta \sigma^2}\})}{\mu R} \}
    \end{align}
    and letting
    \begin{align}
        \Phi = \log(\max\{e, \frac{2 \mu^2 \Delta NKR}{\beta \sigma^2}\})
    \end{align}
    we get 
    \begin{align}
        \text{err}_s \leq c (\Delta \exp(-\frac{R}{C \kappa}) + \frac{\beta \sigma^2 }{\mu^2 N K R} \Phi)
    \end{align}
\end{proof}
\subsection{\lsgd}
\begin{theorem}
    \label{thm:fedavgpl}
    Suppose we run \Lsgd \pcref{algo:fedavg} with a few modifications:
    \begin{enumerate}
        \item Each client performs $\sqrt{K}$ local steps per round
        \item Each local step is computed as $g_{i,k}^{(r)} = \frac{1}{\sqrt{K}} \sum_{b=0}^{\sqrt{K} - 1} \nabla f(x_{i,k}^{(r)}; z_{i,k\sqrt{K} + b}^{(r)})$ where $z_{i,j}^{(r)} \sim \mathcal{D}_i$
        \item In each round, we only sample one client \footnote{This is done for technical reasons--nonconvex analysis of federated learning algorithms like MIME \cite{karimireddy2020mime} require this OR weak convexity to make sure averaging client iterates does not blow up the error.In practice, it has been empirically observed that averaging client weights does not increase the loss \cite{mcmahan2017communication}.  We also provide an analysis for FedAvg that does average clients in \cref{thm:fedavgpl-convergent} that gives up condition number factors.}
    \end{enumerate}
    Then given $\mu$-PL \pcref{asm:pl} of $F$, $\beta$-smoothness of $F_i$'s \pcref{asm:smooth}, $\zeta^2$-heterogeneity of $F_i$'s \pcref{asm:grad_het}, upper bound on initial function suboptimality \pcref{asm:subopt}, and a uniform upper bound of variance $\sigma^2$ \pcref{asm:uniform_variance}, if we choose 
    \begin{align}
        \eta = \frac{1}{\beta}
    \end{align}
    then
    \begin{align}
        \E F(x^{(R)}) - F(x^*) \leq \Delta \exp(-\frac{R\sqrt{K}}{\kappa}) + \frac{\zeta^2}{2 \mu} + \frac{\sigma^2}{2\mu \sqrt{K}}
    \end{align}
    where $K$ is a square number. \footnote{That $K$ is square is assumed for technical simplicity--the proof can be easily generalized.}
\end{theorem}
\begin{proof}

    By smoothness of F \pcref{asm:smooth}, we have for $k \in \{0, \dots, \sqrt{K} - 1\}$
    \begin{align}
        F(x^{(r)}_{i, k+1}) - F(x^{(r)}_{i, k}) \leq - \eta \langle \nabla F(x^{(r)}_{i, k}),  g_{i,k}^{(r)} \rangle + \frac{\beta \eta^2}{2} \|g_{i,k}^{(r)}\|^2
    \end{align}
    Using the fact that for any $a,b$ we have $-2ab = (a-b)^2 - a^2 - b^2$,
    \begin{align}
        F(x^{(r)}_{i, k+1}) - F(x^{(r)}_{i, k}) \leq - \frac{\eta}{2} \|\nabla F(x^{(r)}_{i, k})\|^2 + \frac{\beta \eta^2 - \eta}{2}\| g_{i,k}^{(r)}\|^2 + \frac{\eta}{2} \| g_{i,k}^{(r)} - \nabla F(x^{(r)}_{i, k})\|^2
    \end{align}
    Letting $\eta \leq \frac{1}{\beta}$,
    \begin{align}
        F(x^{(r)}_{k+1}) - F(x^{(r)}_{i,k}) \leq - \frac{\eta}{2} \|\nabla F(x^{(r)}_{i,k})\|^2 + \frac{\eta}{2} \| g_{i,k}^{(r)} - \nabla F(x^{(r)}_{i,k})\|^2
    \end{align}
    Conditioning on everything up to the $k$-th step of the $r$-th round,
    \begin{align}
        \E_{r,k} F(x^{(r)}_{i, k+1}) - F(x^{(r)}_{i,k}) &\leq - \frac{\eta}{2} \|\nabla F(x^{(r)}_{i,k})\|^2 + \frac{\eta}{2} \E_{r,k} \| g_{i,k}^{(r)} - \nabla F(x^{(r)}_{i,k})\|^2 \\
        &\leq - \frac{\eta}{2} \|\nabla F(x^{(r)}_{i,k})\|^2 + \frac{\eta \zeta^2}{2}   + \frac{\eta \sigma^2}{2 \sqrt{K}}
    \end{align}
    Where the last step used the fact that $\E[X^2] = \text{Var}(X) + \E[X]$, the assumption on heterogeneity \pcref{asm:grad_het}, and the assumption on gradient variance \pcref{asm:uniform_variance}.
    Next, using $\mu$-PL of $F$ \pcref{asm:pl},
    \begin{align}
        \E_{r,k} F(x^{(r)}_{i, k+1}) - F(x^{(r)}_{i,k}) \leq - \eta \mu (F(x^{(r)}_{i,k}) - F(x^*)) + \frac{\eta \zeta^2}{2}   + \frac{\eta \sigma^2}{2 \sqrt{K}}
    \end{align}
    which after taking full expectation gives
    \begin{align}
        \E F(x^{(r)}_{i, k+1}) - F(x^*) \leq (1 - \eta \mu)(\E F(x^{(r)}_{i, k}) - F(x^*)) + \frac{\eta \zeta^2}{2} + \frac{\eta \sigma^2}{2 \sqrt{K}}
    \end{align}
    Unrolling the recursion over $k$ we get 
    \begin{align}
        \E F(x^{(r)}_{i, K}) - F(x^*) \leq (1 - \eta \mu)^{\sqrt{K}} (\E F(x^{(r)}_{i,0}) - F(x^*)) + (\frac{\eta \zeta^2}{2 } + \frac{\eta \sigma^2}{2 \sqrt{K}}) \sum_{k=0}^{\sqrt{K}-1} (1 - \eta \mu)^k
    \end{align}
    Recall that $x_{i,K}^{(r)} = x^{(r+1)}$ and $x_{i,0}^{(r)} = x^{(r)}$ because we only sample one client per round.  This gives 
    \begin{align}
        \E F(x^{(r + 1)}) - F(x^*) \leq (1 - \eta \mu)^{\sqrt{K}} (\E F(x^{(r)}) - F(x^*)) + (\frac{\eta \zeta^2}{2 } + \frac{\eta \sigma^2}{2 \sqrt{K}}) \sum_{k=0}^{\sqrt{K}-1} (1 - \eta \mu)^k
    \end{align}
    Unrolling the recursion over $R$, we get
    \begin{align}
        \E F(x^{(R)}) - F(x^*) \leq (1 - \eta \mu)^{R\sqrt{K}} (F(x^{(0)}) - F(x^*)) + (\frac{\eta \zeta^2}{2 } + \frac{\eta \sigma^2}{2 \sqrt{K}}) \sum_{r=0}^{R-1} \sum_{k=0}^{\sqrt{K}-1} (1 - \eta \mu)^{r\sqrt{K} + k}
    \end{align}
    Which can be upper bounded as 
    \begin{align}
        \E F(x^{(R)}) - F(x^*) \leq (1 - \eta \mu)^{R\sqrt{K}} (F(x^{(0)}) - F(x^*)) + \frac{\zeta^2}{2 \mu} + \frac{\sigma^2}{2\mu\sqrt{K}}
    \end{align}
\end{proof}

\subsection{Convergent \lsgd}
\begin{theorem}
    \label{thm:fedavgpl-convergent}
    Suppose we run \Lsgd \pcref{algo:fedavg} with a few modifications:
    \begin{enumerate}
        \item Each client performs $\sqrt{K}$ local steps per round
        \item Each local step is computed as $g_{i,k}^{(r)} = \frac{1}{\sqrt{K}} \sum_{b=0}^{\sqrt{K} - 1} \nabla f(x_{i,k}^{(r)}; z_{i,k\sqrt{K} + b}^{(r)})$ where $z_{i,j}^{(r)} \sim \mathcal{D}_i$
    \end{enumerate}
    Then given $\mu$-PL \pcref{asm:pl} of $F$, $\beta$-smoothness of $F_i$'s \pcref{asm:smooth}, $\zeta^2$-heterogeneity of $F_i$'s \pcref{asm:grad_het}, upper bound on initial function suboptimality \pcref{asm:subopt}, and a uniform upper bound of variance $\sigma^2$ \pcref{asm:uniform_variance}, if we choose 
    \begin{align}
        \eta \leq \frac{1}{\beta}
    \end{align}
    then
    \begin{align}
        \E F(x^{(R)}) - F(x^*) \leq (F(x^{(0)}) - F(x^*))\exp(- \mu \eta R \sqrt{K}) + \frac{\sigma^2}{2  \mu \sqrt{K}} + \frac{\eta^2 \beta^2}{2 \mu } (3 \sqrt{K} \sigma^2  + 6 K  \zeta^2)
    \end{align}
    where $K$ is a square number. \footnote{That $K$ is square is assumed for technical simplicity--the proof can be easily generalized.}
\end{theorem}
\begin{proof}

    By smoothness of F \pcref{asm:smooth}, we have for $k \in \{0, \dots, \sqrt{K} - 1\}$, letting $\bar{x}_{r\sqrt{K} + k} := \frac{1}{N} \sum_{i=1}^N x_{i,k}^{(r)}$
    \begin{align}
        F(\bar{x}_{t+1}) - F(\bar{x}_{t}) \leq - \eta \langle \nabla F(\bar{x}_{t}),  \frac{1}{N} \sum_{i=1}^N g_{i,k}^{(r)} \rangle + \frac{\beta \eta^2}{2} \|\frac{1}{N} \sum_{i=1}^N g_{i,k}^{(r)}\|^2
    \end{align}
    Using the fact that for any $a,b$ we have $-2ab = (a-b)^2 - a^2 - b^2$,
    \begin{align}
        F(\bar{x}_{t+1}) - F(\bar{x}_{t}) \leq - \frac{\eta}{2} \|\nabla F(\bar{x}_{t})\|^2 + \frac{\beta \eta^2 - \eta}{2}\| \frac{1}{N} \sum_{i=1}^N g_{i,k}^{(r)}\|^2 + \frac{\eta}{2} \| \frac{1}{N} \sum_{i=1}^N g_{i,k}^{(r)} - \nabla F(\bar{x}_{t})\|^2
    \end{align}
    Letting $\eta \leq \frac{1}{\beta}$,
    \begin{align}
        F(\bar{x}_{t+1}) - F(\bar{x}_{t}) \leq - \frac{\eta}{2} \|\nabla F(\bar{x}_{t})\|^2 + \frac{\eta}{2} \| \frac{1}{N} \sum_{i=1}^N g_{i,k}^{(r)} - \nabla F(\bar{x}_{t})\|^2
    \end{align}
    Conditioning on everything up to $t$,
    \begin{align}
        \E_t F(\bar{x}_{t+1}) - F(\bar{x}_{t}) &\leq - \frac{\eta}{2} \|\nabla F(\bar{x}_{t})\|^2 + \frac{\eta}{2} \E_t \| \frac{1}{N} \sum_{i=1}^N g_{i,k}^{(r)} - \nabla F(\bar{x}_{t})\|^2 \\
        &\leq - \frac{\eta}{2} \|\nabla F(\bar{x}_{t})\|^2 + \frac{\eta}{2} \E_t \| \frac{1}{N} \sum_{i=1}^N g_{i,k}^{(r)} - \nabla F(\bar{x}_{t})\|^2 \\
        &\leq - \frac{\eta}{2} \|\nabla F(\bar{x}_{t})\|^2 + \frac{\eta \sigma^2}{2 \sqrt{K}} + \frac{\eta}{2} \| \nabla F_i(x_{i,k}^{(r)}) - \nabla F_i (\bar{x}_{t})\|^2 \\
        &\leq - \frac{\eta}{2} \|\nabla F(\bar{x}_{t})\|^2 + \frac{\eta \sigma^2}{2 \sqrt{K}} + \frac{\eta \beta^2}{2} \frac{1}{N} \sum_{i=1}^N \| x_{i,k}^{(r)} - \bar{x}_{t}\|^2
    \end{align}
    Where the second to last step used the fact that $\E[X^2] = \text{Var}(X) + \E[X]^2$, and the assumption on gradient variance \pcref{asm:uniform_variance}, and the last step used the assumption on smoothness \pcref{asm:smooth}.

    From \cite{woodworth2020minibatch} Lemma 8, using the assumption on heterogeneity \pcref{asm:grad_het} 
    \begin{align}
        \frac{1}{N} \sum_{i=1}^N \| x_{i,k}^{(r)} - \bar{x}_{t}\|^2 \leq 3 \sqrt{K} \sigma^2 \eta^2 + 6 K \eta^2 \zeta^2
    \end{align}

    So we have 
    \begin{align}
        \E_t F(\bar{x}_{t+1}) - F(\bar{x}_{t}) &\leq - \frac{\eta}{2} \|\nabla F(\bar{x}_{t})\|^2 + \frac{\eta \sigma^2}{2 \sqrt{K}} + \frac{\eta^3 \beta^2}{2} (3 \sqrt{K} \sigma^2  + 6 K  \zeta^2)
    \end{align}
    Next, using $\mu$-PL of $F$ \pcref{asm:pl},
    \begin{align}
        \E_{t} F(\bar{x}_{t+1}) - F(\bar{x}_{t}) \leq - \eta \mu (F(\bar{x}_{t}) - F(x^*)) + \frac{\eta \sigma^2}{2 \sqrt{K}} + \frac{\eta^3 \beta^2}{2} (3 \sqrt{K} \sigma^2  + 6 K  \zeta^2)
    \end{align}
    which after taking full expectation gives
    \begin{align}
        \E F(\bar{x}_{t+1}) - F(x^*) \leq (1 - \eta \mu)(\E F(\bar{x}_{t}) - F(x^*)) + \frac{\eta \sigma^2}{2 \sqrt{K}} + \frac{\eta^3 \beta^2}{2} (3 \sqrt{K} \sigma^2  + 6 K  \zeta^2)
    \end{align}
    Unrolling the recursion over $k$ we get 
    \begin{align}
        \E F(x^{(r+1)}) - F(x^*) \leq (1 - \eta \mu)^{\sqrt{K}} (\E F(x^{(r)}) - F(x^*)) + (\frac{\eta \sigma^2}{2 \sqrt{K}} + \frac{\eta^3 \beta^2}{2} (3 \sqrt{K} \sigma^2  + 6 K  \zeta^2)) \sum_{k=0}^{\sqrt{K}-1} (1 - \eta \mu)^k
    \end{align}
    Unrolling the recursion over $R$, we get
    \begin{align}
        & \E F(x^{(R)}) - F(x^*) \\
        & \ \ \ \ \leq (1 - \eta \mu)^{R\sqrt{K}} (F(x^{(0)}) - F(x^*)) + (\frac{\eta \sigma^2}{2 \sqrt{K}} + \frac{\eta^3 \beta^2}{2} (3 \sqrt{K} \sigma^2  + 6 K  \zeta^2)) \sum_{r=0}^{R-1} \sum_{k=0}^{\sqrt{K}-1} (1 - \eta \mu)^{r\sqrt{K} + k}
    \end{align}
    Which can be upper bounded as 
    \begin{align}
        \E F(x^{(R)}) - F(x^*) &\leq (1 - \eta \mu)^{R\sqrt{K}} (F(x^{(0)}) - F(x^*)) + \frac{\sigma^2}{2  \mu \sqrt{K}} + \frac{\eta^2 \beta^2}{2 \mu } (3 \sqrt{K} \sigma^2  + 6 K  \zeta^2) \\
        &\leq  (F(x^{(0)}) - F(x^*))\exp(- \mu \eta R \sqrt{K}) + \frac{\sigma^2}{2  \mu \sqrt{K}} + \frac{\eta^2 \beta^2}{2 \mu } (3 \sqrt{K} \sigma^2  + 6 K  \zeta^2)
    \end{align}
\end{proof}
\subsection{M-\Lsgd}
\begin{theorem}
    \label{thm:pl-m-lsgd}
    Suppose we run M-\lsgd \pcref{algo:m-lsgd} with a few modifications:
    \begin{enumerate}
        \item Each client performs $\sqrt{K}$ local steps per round
        \item Each local step is computed as $g_{i,k}^{(r)} = \frac{1}{\sqrt{K}} \sum_{b=0}^{\sqrt{K} - 1} \nabla f(x_{i,k}^{(r)}; z_{i,k\sqrt{K} + b}^{(r)})$ where $z_{i,j}^{(r)} \sim \mathcal{D}_i$
    \end{enumerate}
    Then given $\mu$-PL \pcref{asm:pl} of $F$, $\beta$-smoothness of $F_i$'s \pcref{asm:smooth}, $\zeta^2$-heterogeneity of $F_i$'s \pcref{asm:grad_het}, upper bound on initial function suboptimality \pcref{asm:subopt}, and a uniform upper bound of variance $\sigma^2$ \pcref{asm:uniform_variance}, if we choose 
    \begin{align}
        \eta = \min \{\frac{1}{\beta}, \frac{\log( \max \{e, \frac{2 \Delta  \mu^3 R^2 K}{(3 \sqrt{K} \sigma^2 + 6 K \zeta^2)}\})}{\mu R \sqrt{K}} \}
    \end{align}
    and $\eta_s = \frac{\eta}{2^s}$ and $R_s = \frac{2^s \log (4)}{\mu \eta \sqrt{K}}$ then
    \begin{align}
        \E F(x^{(s, R_s)}) - F(x^*) \leq \frac{1}{2^{s}}(\Delta \exp(-\frac{R \sqrt{K}}{\kappa}) + \frac{\beta^2}{2 \mu^3 R^2 K}(3 \sqrt{K} \sigma^2 + 6 K \zeta^2)) +  \frac{\sigma^2}{2 \mu \sqrt{K}} \sum_{j=0}^{s} \frac{1}{2^j}
    \end{align}
    and if $s$ is a constant along with $K \geq \kappa^2$,
    then 
    \begin{align}
        \E F(x^{(s, R_s)}) - F(x^*) \leq c(\Delta \exp(-\frac{R \sqrt{K}}{C \kappa}) + (3 \sqrt{K} \sigma^2 + 6 K \zeta^2) \frac{\beta^2}{2 \mu^3 R^2 K} \Phi^2 ) + \frac{\sigma^2}{2\mu \sqrt{K}}
    \end{align}
    for some universal constant $c,C$
    where $K$ is a square number. \footnote{That $K$ is square is assumed for technical simplicity--the proof can be easily generalized.}
\end{theorem}
\begin{proof}
    Let 
    \begin{align}
        \text{err}_s = \E F(x^{(s, R_s)}) - F(x^*)
    \end{align}
    We want to prove the following inductive hypothesis for all $s$:
    \begin{align}
        \text{err}_s \leq \frac{1}{2^{s-1}}(\Delta \exp(-\mu \eta R_1 \sqrt{K}) + \frac{\eta^2 \beta^2}{2 \mu}(3 \sqrt{K} \sigma^2 + 6 K \zeta^2)) + \frac{\sigma^2}{2 \mu \sqrt{K}} \sum_{j=0}^{s-1} \frac{1}{2^j}
    \end{align}
    We start with the base case: $\eta_1 = \eta$.  Then we of course have \pcref{thm:fedavgpl-convergent}
    \begin{align}
        \text{err}_1 \leq \Delta \exp(- \mu \eta R_1 \sqrt{K})  + \frac{\eta^2 \beta^2}{2 \mu } (3 \sqrt{K} \sigma^2  + 6 K  \zeta^2) + \frac{\sigma^2}{2  \mu \sqrt{K}}
    \end{align}
    The inductive case and the rest of the proof is similar to that of \cref{thm:pl-m-sgd}.
    Now we look at the inductive case.  Then using that $\eta_s = \frac{\eta}{2^s}$ and $R_s = \frac{2^s \log (4)}{\mu \eta \sqrt{K}}$,
    \begin{align}
        \text{err}_{s+1} &\leq \text{err}_s \exp(-\mu \eta_s R_s \sqrt{K}) + \frac{\sigma^2}{2  \mu \sqrt{K}} + \frac{\eta_s^2 \beta^2}{2 \mu } (3 \sqrt{K} \sigma^2  + 6 K  \zeta^2) \\
        &\leq (\frac{1}{2^{s-1}}(\Delta \exp(-\mu \eta R_1 \sqrt{K}) + \frac{\eta^2 \beta^2}{2 \mu}(3 \sqrt{K} \sigma^2 + 6 K \zeta^2)) + \frac{\sigma^2}{2 \mu \sqrt{K}} \sum_{j=0}^{s-1} \frac{1}{2^j})(\frac{1}{4}) \\
        & \ \ \ + \frac{\sigma^2}{2  \mu \sqrt{K}} + \frac{\eta^2 \beta^2}{2 \mu 2^{s + 1}} (3 \sqrt{K} \sigma^2  + 6 K  \zeta^2) \\
        &\leq \frac{1}{2^{s}}(\Delta \exp(-\mu \eta R_1 \sqrt{K}) + \frac{\eta^2 \beta^2}{2 \mu}(3 \sqrt{K} \sigma^2 + 6 K \zeta^2)) +  \frac{\sigma^2}{2 \mu \sqrt{K}} \sum_{j=0}^{s} \frac{1}{2^j}
    \end{align}
    Which completes the induction.
    If $s$ is a constant and $K \geq \kappa^2$, then
    \begin{align}
        \text{err}_s \leq c (\Delta \exp(-\mu \eta (R/C) \sqrt{K}) + \frac{\eta^2 \beta^2}{2 \mu}(3 \sqrt{K} \sigma^2 + 6 K \zeta^2)) + \frac{\sigma^2}{2\mu \sqrt{K}}
    \end{align}
    for a universal constant $c, C$.
    If we choose 
    \begin{align}
        \eta = \min \{\frac{1}{\beta}, \frac{\log( \max \{e, \frac{2 \Delta  \mu^3 R^2 K}{(3 \sqrt{K} \sigma^2 + 6 K \zeta^2)}\})}{\mu R \sqrt{K}} \}
    \end{align}
    This gives 
    \begin{align}
        \text{err}_s \leq c'(\Delta \exp(-\frac{R \sqrt{K}}{C \kappa}) + (3 \sqrt{K} \sigma^2 + 6 K \zeta^2) \frac{\beta^2}{2 \mu^3 R^2 K} \Phi^2 ) + \frac{\sigma^2}{2\mu \sqrt{K}}
    \end{align}
    where 
    \begin{align}
        \Phi = \log( \max \{e, \frac{2 \Delta  \mu^3 R^2 K}{(3 \sqrt{K} \sigma^2 + 6 K \zeta^2)}\})
    \end{align}
    and $c'$ is a universal constant.
\end{proof}
\subsection{\lsgd $\to$ \mbsgd}
\begin{theorem}
    \label{thm:pl-lsgd-sgd}
    Suppose we run \cref{algo:chaining} where:
    \begin{enumerate}
        \item $\ahead$ is \Lsgd \pcref{algo:fedavg} under the setting of \cref{thm:fedavgpl}, run for $R$ rounds
        \item $\atail$ is \mbsgd \pcref{algo:mbsgd} under the setting of \cref{thm:plsgd}, run for $R$ rounds
    \end{enumerate}
    If we additionally assume that loss queries have variance bounded by $\sigma^2$ \pcref{asm:cost_variance}, then we have convergence rate 
    \begin{align}
        \E F(\hat{x}_2) - F(x^*) \leq (\min \{\Delta \exp(-\frac{R\sqrt{K}}{\kappa}) + \frac{\zeta^2}{2 \mu} + \frac{\sigma^2}{2\mu \sqrt{K}}, \Delta \} + \frac{4\sigma}{\sqrt{N K}}) \exp(-\frac{R}{\kappa}) + \frac{\beta \sigma^2}{\mu^2 N K R} \Phi
    \end{align}
    Where
    \begin{align}
        \Phi := \log(\max\{e, \frac{2 \mu^2 \Delta NKR}{\beta \sigma^2}\})
    \end{align}
\end{theorem}
\begin{proof}
    This is the same as the proof for \cref{thm:lsgd-sgd}.
\end{proof}
\subsection{M-\lsgd $\to$ M-\mbsgd}
\begin{theorem}
    \label{thm:pl-mlsgd-msgd}
    Suppose we run \cref{algo:chaining} where:
    \begin{enumerate}
        \item $\ahead$ is M-\Lsgd \pcref{algo:m-lsgd} under the setting of \cref{thm:pl-m-lsgd}, run for $R$ rounds
        \item $\atail$ is M-\mbsgd \pcref{algo:m-mbsgd} under the setting of \cref{thm:pl-m-sgd}, run for $R$ rounds
    \end{enumerate}
    If we additionally assume that loss queries have variance bounded by $\sigma^2$ \pcref{asm:cost_variance}, then we have convergence rate 
    \begin{align}
        & \ \ \E F(\hat{x}_2) - F(x^*) \\
        &\leq c'( (\min \{c(\Delta \exp(-\frac{R \sqrt{K}}{C \kappa}) + (3 \sqrt{K} \sigma^2 + 6 K \zeta^2) \frac{\beta^2}{2 \mu^3 R^2 K} \Phi^2 ) + \frac{\sigma^2}{2\mu \sqrt{K}}, \Delta \} + \frac{4\sigma}{\sqrt{N K}}) \exp(-\frac{R}{C' \kappa}) \\
        & \ \ \ + \frac{\beta \sigma^2}{\mu^2 N K R} \Phi')
    \end{align}
    Where
    \begin{align}
        \Phi = \log( \max \{e, \frac{2 \Delta  \mu^3 R^2 K}{(3 \sqrt{K} \sigma^2 + 6 K \zeta^2)}\})
    \end{align}
    \begin{align}
        \Phi' = \log(\max\{e, \frac{2 \mu^2 \Delta NKR}{\beta \sigma^2}\})
    \end{align}
    and $c,c',C, C'$ are absolute constants.
\end{theorem}
\begin{proof}
    After running $\ahead$ where $\ahead$ is M-\Lsgd under the setting of \cref{thm:pl-m-lsgd}, we have that with absolute constants $c, C$ and 
    \begin{align}
        \Phi = \log( \max \{e, \frac{2 \Delta  \mu^3 R^2 K}{(3 \sqrt{K} \sigma^2 + 6 K \zeta^2)}\})
    \end{align}
    we have
    \begin{align}
        \E F(\hat{x}_{1/2}) - F(x^*) \leq c(\Delta \exp(-\frac{R \sqrt{K}}{C \kappa}) + (3 \sqrt{K} \sigma^2 + 6 K \zeta^2) \frac{\beta^2}{2 \mu^3 R^2 K} \Phi^2 ) + \frac{\sigma^2}{2\mu \sqrt{K}}
    \end{align}
    By \cref{lemma:choosefunc}, we know that under \cref{asm:cost_variance}, we have 
    \begin{align}
        \E F(\hat{x}_1) - F(x^*) &\leq \min \{\E F(\hat{x}_{1/2}) - F(x^*), \E F(\hat{x}_{0}) - F(x^*)\} + \frac{4\sigma}{\sqrt{N K}} \\
        &\leq \min \{c(\Delta \exp(-\frac{R \sqrt{K}}{C \kappa}) + (3 \sqrt{K} \sigma^2 + 6 K \zeta^2) \frac{\beta^2}{2 \mu^3 R^2 K} \Phi^2 ) + \frac{\sigma^2}{2\mu \sqrt{K}}, \Delta \} + \frac{4\sigma}{\sqrt{N K}}
    \end{align}
    Now we run $\atail$ as \mbsgd \pcref{algo:mbsgd} under the setting of \cref{thm:strongsgd} using $\hat{x}_1$ is the initialization, which gives
    \begin{align}
        \E F(\hat{x}_2) - F(x^*) \leq c' ((\E F(\hat{x}_1) - F(x^*)) \exp(-\frac{R}{C' \kappa}) + \frac{\beta \sigma^2 }{\mu^2 N K R} \Phi')
    \end{align}
    where $c',C'$ are absolute constants and 
    \begin{align}
        \Phi' = \log(\max\{e, \frac{2 \mu^2 \Delta NKR}{\beta \sigma^2}\})
    \end{align}
    which gives the convergence rate
    \begin{align}
        & \ \ \E F(\hat{x}_2) - F(x^*) \\
        &\leq c'( (\min \{c(\Delta \exp(-\frac{R \sqrt{K}}{C \kappa}) + (3 \sqrt{K} \sigma^2 + 6 K \zeta^2) \frac{\beta^2}{2 \mu^3 R^2 K} \Phi^2 ) + \frac{\sigma^2}{2\mu \sqrt{K}}, \Delta \} + \frac{4\sigma}{\sqrt{N K}}) \exp(-\frac{R}{C' \kappa}) \\
        & \ \ \ + \frac{\beta \sigma^2}{\mu^2 N K R} \Phi')
    \end{align}
\end{proof}
