# Supplementary material for: FedChain: Chained Algorithms for Near-Optimal Communication Cost in Federated Learning
Source: arXiv:2108.06869 source file (2023-04-16)
Supplement: Supplementary file 4 [file strongproofs.tex]

%!TEX root = ./main.tex
\section{Proofs under strong convexity}
\subsection{SAGA}
The update is as follows:
\begin{align}
    \x{r+1} = \x{r} - \eta (\frac{1}{S} \sum_{i \in \mathcal{S}_r} [\frac{1}{K}\sum_{k =0}^{K-1} \nabla f(\x{r}; z_{i,k}^{(r)}) - c_i^{(r)}] + c^{(r)})
\end{align}
where we have that 
\begin{align}
    \tilde{c}_i^{(r+1)} = \frac{1}{K} \sum_{k=0}^{K-1}\nabla f(\x{r}; z_{i,k}^{(r)})
\end{align}
and 
\begin{align}
    c_i^{(r+1)} = \begin{cases}
        \tilde{c}_i^{(r+1)} \text{ if } i \in \mathcal{S}_r \\
        c_i^{(r)} \text{ otherwise}
    \end{cases}
\end{align}
and finally 
\begin{align}
    c^{(r+1)} = \frac{1}{N}\sum_{i=1}^N c_i^{(r+1)}
\end{align}
To simplify notation, let \[g^{(r)} := (\frac{1}{S} \sum_{i \in \mathcal{S}_r} [\frac{1}{K}\sum_{k =0}^{K-1} \nabla f(\x{r}; z_{i,k}^{(r)}) - c_i^{(r)}] + c^{(r)})\]
and let the control lag be 
\begin{align}
    \mathcal{C}_r = \frac{1}{N} \sum_{i=1}^N \E \|\nabla F_i(x^*) - \E c_i^{(r)}\|^2
\end{align}
\begin{proof}
    Following the standard analysis,
    \begin{align}
        &\E_{r} \|\x{r+1} - x^*\|^2 \\
        &= \|\x{r} - x^*\|^2 -  2 \eta\E_r \langle g^{(r)}, \x{r} - x^* \rangle + \E_r \|\eta g^{(r)} \|^2 \\
    \end{align}
    We treat each of these terms separately.
    
\textbf{Second term:}
    Observe first that 
    \begin{align}
        \E_r g^{(r)} &= \E_r(\frac{1}{S} \sum_{i \in \mathcal{S}_r} [\frac{1}{K}\sum_{k =0}^{K-1} \nabla f(\x{r}; z_{i,k}^{(r)}) - c_i^{(r)}] + c^{(r)}) \\
        &= \nabla F(\x{r})
    \end{align}
    And so the middle term has, by (strong) convexity,
    \begin{align}
        -  2 \eta\E_r \langle g^{(r)}, \x{r} - x^* \rangle &= - 2 \eta \langle \nabla F(\x{r}), \x{r} - x^* \rangle \\
        &\leq-2 \eta (F(\x{r}) - F(x^*) + \frac{\mu}{2} \|\x{r} - x^*\|^2)
    \end{align}
\textbf{Third term:}
\begin{align}
    &\E_r \|\eta g^{(r)}\|^2 \\
    &= \E_r \| \eta (\frac{1}{S} \sum_{i \in \mathcal{S}_r} [\frac{1}{K}\sum_{k =0}^{K-1} \nabla f(\x{r}; z_{i,k}^{(r)}) - c_i^{(r)}] + c^{(r)})\|^2 \\
    &= \eta^2 \E_r \|\frac{1}{KS} \sum_{k, i \in \mathcal{S}_r} \nabla f(\x{r}; z_{i,k}^{(r)}) - c_i^{(r)} + c^{(r)}\|^2 \\
    &\leq 4 \eta^2 \E_r \|\frac{1}{KS} \sum_{k, i \in \mathcal{S}_r} \nabla f(\x{r}; z_{i,k}^{(r)}) - \nabla F_i(\x{r})\|^2 + 4 \eta^2 \E_r \|c^{(r)}\|^2 \\
    & \ \ \ \ + 4 \eta^2 \E_r \|\frac{1}{KS} \sum_{k, i \in \mathcal{S}_r} \nabla F_i(x^*) - c_i^{(r)}\|^2 + 4 \eta^2 \E_r \|\frac{1}{KS} \sum_{k, i \in \mathcal{S}_r} \nabla F_i(\x{r}) - \nabla F_i(x^*)\|^2 \\
\end{align}
Where the last inequality comes from the relaxed triangle inequality.  Then, by using \cref{asm:uniform_variance}, \cref{asm:smooth}, and \cref{asm:convex},
\begin{align}
    &\E_r \|\eta g^{(r)}\|^2 \\
    &\leq 4 \eta^2 \E_r \|c^{(r)}\|^2  + 4 \eta^2 \E_r \|\frac{1}{KS} \sum_{k, i \in \mathcal{S}_r} \nabla F_i(x^*) - c_i^{(r)}\|^2 + 8 \beta \eta^2 [F(\x{r}) - F(x^*)] + \frac{4 \eta^2 \sigma^2}{KS}
\end{align}
Taking full expectation and separating out the variance of the control variates,
\begin{align}
    &\E \|\eta g^{(r)}\|^2 \\
    &\leq 4 \eta^2 \|\E c^{(r)}\|^2  + 4 \eta^2 \|\frac{1}{KS} \sum_{k, i \in \mathcal{S}_r} \nabla F_i(x^*) - \E c_i^{(r)}\|^2 + 8 \beta \eta^2 [F(\x{r}) - F(x^*)] + \frac{12 \eta^2 \sigma^2}{KS}
\end{align}
Now observe that because $c^{(r)} = \frac{1}{N} \sum_{i =1}^N c_i^{(r)}$,
\begin{align}
    \E \|\eta g^{(r)}\|^2 
    &\leq \frac{8 \eta^2}{N} \sum_{i=1}^N \| \nabla F_i(x^*) - \E c_i^{(r)}\|^2 + 8 \beta \eta^2 [F(\x{r}) - F(x^*)] + \frac{12 \eta^2 \sigma^2}{KS} \\
    &\leq 8 \eta^2\mathcal{C}_r + 8 \beta \eta^2 [F(\x{r}) - F(x^*)] + \frac{12 \eta^2 \sigma^2}{KS} 
\end{align}

\textbf{Bounding the control lag: }

Recall that 
\begin{align}
    c_i^{(r+1)} = \begin{cases}
        c_i^{(r)} \text{ w.p. } 1 - \frac{S}{N}\\
        \frac{1}{K} \sum_{k=0}^{K-1} \nabla f(\x{r}; z_{i,k}^{(r)}) \text{ w.p. } \frac{S}{N}
    \end{cases}
\end{align}
Therefore
\begin{align}
    \E c_i^{(r+1)} = (1 - \frac{S}{N}) \E[c_i^{(r)}] + \frac{S}{N} \E \nabla F_i(\x{r})
\end{align}
Returning to the definition of $\mathcal{C}_{r + 1}$,
\begin{align}
    \mathcal{C}_{r+1} &= \frac{1}{N} \sum_{i=1}^N \E \| \E[c_i^{(r+1)}] - \nabla F_i(x^*)\|^2 \\
    &= \frac{1}{N} \sum_{i=1}^N \E \| (1 - \frac{S}{N}) (\E[c_i^{(r)}] - \nabla F_i(x^*)) + \frac{S}{N} (\E \nabla F_i(\x{r}) - \nabla F_i(x^*))\|^2 \\
    &\leq (1 - \frac{S}{N}) \mathcal{C}_r + \frac{S}{N^2} \sum_{i=1}^N \E \|\nabla F_i(\x{r}) - \nabla F_i(x^*)\|^2
\end{align}
where in the last inequality we applied Jensen's inequality twice.  By smoothness of $F_i$'s \pcref{asm:smooth},
\begin{align}
    \mathcal{C}_{r+1} \leq (1 - \frac{S}{N}) \mathcal{C}_r + \frac{2\beta S}{N}[\E F(\x{r}) - F(x^*)]
\end{align}
\textbf{Putting it together: }

So putting it all together, we have
\begin{align}
    \E \|\x{r+1} - x^*\|^2 \leq (1 - \eta \mu)\E \|\x{r} - x^*\|^2 -\eta(2 - 8 \beta \eta) (F(\x{r}) - F(x^*)) + 8 \eta^2\mathcal{C}_r + \frac{12 \eta^2 \sigma^2}{KS} 
\end{align}
From our bound on the control lag,
\begin{align}
    \frac{9 \eta^2 N}{S} \mathcal{C}_{r+1} &\leq \frac{9 \eta^2 N}{S} (1 - \frac{S}{N}) \mathcal{C}_r + 18\beta \eta^2[\E F(\x{r}) - F(x^*)] \\
    &= (1 - \eta \mu)\frac{9\eta^2 N}{S}\mathcal{C}_r + 9\eta^2 (\frac{\eta \mu N}{S} - 1)\mathcal{C}_r + 18\beta \eta^2[\E F(\x{r}) - F(x^*)]
\end{align}
Adding both inequalities, we have 
\begin{align}
    &\E \|\x{r+1} - x^*\|^2 + \frac{9 \eta^2 N}{S} \mathcal{C}_{r+1} \\
    &\leq (1 - \eta \mu)[\E \|\x{r} - x^*\|^2 + \frac{9\eta^2 N}{S}\mathcal{C}_r] - \eta (2 - 26 \beta \eta)(\E F(\x{r}) - F(x^*)) + \eta^2 (\frac{9 \eta \mu N}{S} - 1) \mathcal{C}_r + \frac{12 \eta^2 \sigma^2}{KS}
\end{align}
Let $\eta \leq \frac{1}{26 \beta}$, $\eta \leq \frac{S}{9 \mu N}$, then 
\begin{align}
    \label{eq:saga-recurrence}
    \E \|\x{r+1} - x^*\|^2 + \frac{9 \eta^2 N}{S} \mathcal{C}_{r+1} 
    &\leq (1 - \eta \mu)[\E \|\x{r} - x^*\|^2 + \frac{9\eta^2 N}{S}\mathcal{C}_r] - \eta (\E F(\x{r}) - F(x^*))  + \frac{12 \eta^2 \sigma^2}{KS}
\end{align}
Then by using Lemma 1 in \citep{karimireddy2020scaffold}, setting $\eta_{\text{max}} = \min \{\frac{1}{26 \beta}, \frac{S}{9 \mu N}\}$, $R \geq \frac{1}{2 \eta_\text{max} \mu}$, and choosing $\eta = \min \{\frac{\log(\max(1, \mu^2 R d_0/c))}{\mu R}, \eta_{\max} \}$ where $d_0 = \E \|\x{0} - x^*\|^2 + \frac{9 N \eta^2}{S} \mathcal{C}_0$ and $c = \frac{12 \sigma^2}{KS}$, we have that by outputting $\hat{x} = \frac{1}{W_R} \sum_{r=0}^{R} w_r \x{r}$ with $W_R = \sum_{r=0}^{R} w_r$ and $w_r = (1 - \mu \eta)^{1-r}$, we have

\begin{align}
    \E F(\hat{x}) - F(x^*) &\leq \tilde{\mathcal{O}}(\mu d_0 \exp(-\mu \eta_{\max} R) + \frac{c}{\mu R}) \\
    &= \tilde{\mathcal{O}}(\mu d_0 \exp(-\mu \eta_{\max} R) + \frac{c}{\mu R}) \\
    &= \tilde{\mathcal{O}}(\mu [\E \|\x{0} - x^*\|^2 + \frac{N \eta^2}{S} \mathcal{C}_0] \exp(-\mu \eta_{\max} R) + \frac{\sigma^2}{\mu R K S})
\end{align}

% \textbf{Option 1: } We use a warm-start strategy to initialize all control variates in the first $N/S$ rounds such that \[c_i^{(0)} = \frac{1}{K} \sum_{k=0}^{K-1} \nabla f(\x{0}; z_{i,k}^{-1})\]

% By smoothness of $F_i$'s \pcref{asm:smooth},
% \begin{align}
%     \mathcal{C}_0 = \frac{1}{N} \sum_{i=1}^N \E \|\E c_i^{(0)} - \nabla F_i(x^*)\|^2 = \frac{1}{N} \sum_{i=1}^N \E \|\nabla F_i(\x{0}) - \nabla F_i(x^*)\|^2 
%     \leq  \beta \E(F(\x{0}) - F(x^*))
% \end{align}
% And recalling that $\eta \leq \min \{\frac{1}{26 \beta}, \frac{S}{9 \mu N}\}$, we know that 
% \begin{align}
%     \frac{9N \eta^2}{S} \mathcal{C}_0 &\leq \frac{9N \eta^2}{S} \beta \E (F(\x{0}) - F(x^*)) \leq \frac{\eta \beta}{\mu}(F(\x{0}) - F(x^*)) \leq \frac{1}{\mu} \Delta  
% \end{align}
% we also know that by strong convexity \cref{asm:strongconvex},
% \begin{align}
%     \E \| \x{0} - x^*\|^2 \leq \frac{1}{\mu} \Delta
% \end{align}
% So altogether
% \begin{align}
%     \E F(\hat{x}) - F(x^*) \leq \tilde{\mathcal{O}}(\Delta \exp(-\min \{\frac{\mu}{26 \beta}, \frac{S}{9 N}\}  R) + \frac{\sigma^2}{\mu R K S})
% \end{align}

Observe that all $c_i^{(0)}$'s are initialized at zero, so:
\begin{align}
    c_i^{(0)} = 0
\end{align}
Then we have that 
\begin{align}
    \mathcal{C}_0 = \frac{1}{N} \sum_{i=1}^N \|\nabla F_i(x^*)\|^2 = \zeta_*^2
\end{align}
Which implies
\begin{align}
    \frac{9N \eta^2}{S} \mathcal{C}_0 \leq \min\{\frac{\zeta_*^2}{26 \beta \mu}, \frac{N \zeta_*^2}{S \beta^2}\}
\end{align}

% Now, we use the first $N/S$ rounds to initialize $c_i^{(0)} = \frac{1}{K} \sum_{k=0}^{K-1} \nabla f(x^{(0)}; z_{i,k}^{(-1)})$.  This gets
% \begin{align}
%     \frac{\eta^2 N}{S}\E \mathcal{C}_0 &\leq \tilde{\mathcal{O}}(\frac{1}{\beta \mu} \frac{1}{N} \sum_{i=1}^N \E \|\nabla F_i(x^{(0)}) - \nabla F_i(x^*)\|^2 + \frac{\sigma^2}{K \beta \mu}) \\ 
%     &\leq \tilde{\mathcal{O}}(\kappa \E \|x^{(0)} - x^*\|^2 + \frac{\sigma^2}{K \beta \mu})
% \end{align}
% Choosing $K \geq \frac{\mu^2}{\sigma^2 D^2}$,
% \begin{align}
%     \frac{\eta^2 N}{S}\E \mathcal{C}_0 &\leq \tilde{\mathcal{O}}(\frac{1}{\beta \mu} \frac{1}{N} \sum_{i=1}^N \E \|\nabla F_i(x^{(0)}) - \nabla F_i(x^*)\|^2 + \frac{\sigma^2}{K \beta \mu}) \\ 
%     &\leq \tilde{\mathcal{O}}(\kappa D^2)
% \end{align}
This gives
\begin{align}
    \E F(\hat{x}) - F(x^*) \leq \tilde{\mathcal{O}}((\Delta  + \frac{\zeta_*^2}{\beta})\exp(-\min \{\frac{1}{26 \kappa}, \frac{S}{9 N}\}  R) + \frac{\sigma^2}{\mu R K S}) 
\end{align}

On the other hand, from the recurrence \cref{eq:saga-recurrence}, we see that 
\begin{align}
    \E \|x^{(R)} - x^*\|^2 \leq \tilde{\mathcal{O}}((\E\|x^{(0)} - x^*\|^2 + \frac{N \zeta_*^2}{S \beta^2})\exp(-\eta \mu R) + \frac{\eta \sigma^2}{\mu KS})
\end{align}
Given the stepsize choice, as well as $K \geq \frac{SR \mu^2}{\sigma^2 D^2}$
\begin{align}
    \E \|x^{(R)} - x^*\|^2 \leq \tilde{\mathcal{O}}(D^2+ \frac{N \zeta_*^2}{S \beta^2})
\end{align}
% On the other hand, we also have that 
% \begin{align}
%     \E F(\hat{x}) - F(x^*) &\leq \frac{D^2 + \frac{9 \eta^2 N}{S} \mathcal{C}_0}{\eta W_R} + \frac{12 \eta \sigma^2}{KS} \leq \frac{D^2 + \frac{9 \eta^2 N}{S} \mathcal{C}_0}{\eta} \exp(-\mu \eta R) + \frac{12 \eta \sigma^2}{KS} \\
%     &\leq (\beta D^2 + \frac{\zeta_*^2}{\mu} + \frac{9 D^2 \mu N}{ S} + \frac{\zeta^2_* N}{\beta  S})\exp(-\mu \eta R) + \frac{12 \eta \sigma^2}{KS}
% \end{align}
% Setting $\tilde{D}^2 = \beta D^2 + \frac{\zeta_*^2}{\mu} + \frac{9 D^2 \mu N}{ S} + \frac{\zeta^2_* N}{\beta  S}$,
% we set $\eta = \min \{\frac{\log(\max(1, \mu R \tilde{D}^2/(\sigma^2/KS)))}{\mu R}, \frac{1}{26 \beta}, \frac{S}{9 \mu N}\}$
% Which gives us 
% \begin{align}
%     \E F(\hat{x}) - F(x^*) \leq \tilde{\mathcal{O}}((\beta D^2 + \frac{\zeta_*^2}{\mu} + \frac{9 D^2 \mu N}{ S} + \frac{\zeta^2_* N}{\beta  S})\exp(-\min \{\kappa^{-1}, \frac{S}{N}\} R) + \frac{\sigma^2}{\mu S K R})
% \end{align}
\end{proof}
\subsection{Smoothed SAGA}
\begin{proof}
    Recall from the proof of SAGA that the solution satisfies, if $R > 52 \frac{\beta + \mu}{\mu}$ and $R > \frac{18 N}{S} $,
    \begin{align}
        \E F_\mu(\hat{x}) - F_\mu(x^*_\mu) \leq \tilde{\mathcal{O}}(\Delta  \exp(-\min \{\frac{\mu}{26(\beta + \mu)}, \frac{S}{9 N}\}  R) +  \frac{\zeta_*^2}{\beta + \mu}\exp(-\min \{\frac{\mu}{26(\beta + \mu)}, \frac{S}{9N}\}  R) + \frac{\sigma^2}{\mu R K S}) 
    \end{align}
    From \cref{lemma:suboptupper}, we know that 
    \begin{align}
        \E \|\nabla F(\hat{x})\|^2 &\leq \tilde{\mathcal{O}}(\beta \Delta \exp(-\min \{\frac{\mu}{26(\beta + \mu)}, \frac{S}{9 N}\}  R) \\
        &+ \zeta_*^2\exp(-\min \{\frac{\mu}{26(\beta + \mu)}, \frac{S}{9N}\}  R) + \frac{(\beta + \mu)\sigma^2}{\mu R K S} + \mu \Delta)
    \end{align}
    We choose $K > \frac{R S}{(\beta + \mu)\sigma^2 \Delta}$ to get
    \begin{align}
        \E \|\nabla F(\hat{x})\|^2 &\leq \tilde{\mathcal{O}}(\beta \Delta \exp(-\min \{\frac{\mu}{26(\beta + \mu)}, \frac{S}{9 N}\}  R) + \zeta_*^2\exp(-\min \{\frac{\mu}{26(\beta + \mu)}, \frac{S}{9N}\}  R) + \mu \Delta)
    \end{align} 
    If we choose 
    \begin{align}
        \mu = \frac{104 \beta}{R} \log(e + R)
    \end{align}
    The constraint that $R > 52 \frac{\beta + \mu}{\mu}$ is always satisfied, and 
    \begin{align}
        \E \|\nabla F(\hat{x})\|^2 &\leq \tilde{\mathcal{O}}(\beta \Delta \exp(-\min \{\frac{4 \log(e + R)}{R}, \frac{S}{9 N}\}  R) + \zeta_*^2\exp(-\min \{\frac{4 \log(e + R)}{R}, \frac{S}{9N}\}  R) + \frac{\beta \Delta}{R})
    \end{align} 
    If $\frac{S}{9N} < \frac{4 \log (e + R)}{R}$, then we have 
    \begin{align}
        \E \|\nabla F(\hat{x})\|^2 &\leq \tilde{\mathcal{O}}(\beta \Delta \exp(-\frac{S}{9 N} R) + \zeta_*^2\exp(-\frac{S}{9N}  R) + \frac{\beta \Delta}{R})
    \end{align}
    Otherwise, we have 
    \begin{align}
        \E \|\nabla F(\hat{x})\|^2 &\leq \tilde{\mathcal{O}}(\frac{\zeta_*^2}{R} + \frac{\beta \Delta}{R})
    \end{align} 
    Given that $R > \frac{18 N}{S}$, we have that overall,
    \begin{align}
        \E \|\nabla F(\hat{x})\|^2 &\leq \tilde{\mathcal{O}}(\frac{\zeta_*^2}{R} + \frac{\beta \Delta}{R})
    \end{align}
\end{proof}

\subsection{SSNM}
\newcommand{\ir}{i_r}
\newcommand{\yr}{y_{\ir}^{(r)}}
\newcommand{\Fr}{\tilde{F}_{\ir}}
\newcommand{\phir}{\phi_{\ir}^{(r)}}
\newcommand{\gr}{g^{(r)}}
Most of this proof follows that of \citep{zhou2019direct} Theorem 1.

\textbf{Variance Bound: }

\begin{align}
    &\E_{\mathcal{S}_r} [\|g^{(r)} - \frac{1}{N} \sum_{i=1}^N \nabla \tilde{F}_i(y_{i_r}^{(r)})\|^2] \\
    &\leq \E_{\mathcal{S}_r} \|\frac{1}{S} \sum_{i_r \in \mathcal{S}_r} \nabla \tilde{F}_{\ir}(y_{\ir}^{(r)}) - \nabla \tilde{F}_{\ir}(\phi_{i_r}^{(r)}) - \frac{1}{N} \sum_{i=1}^N (\nabla \tilde{F}_i(y_{i}^{(r)}) - \nabla \tilde{F}_i(\phi_{i}^{(r)}))\|^2 + \frac{\sigma^2}{KS} \\
    &\leq \E_{\mathcal{S}_r} \|\frac{1}{S} \sum_{i_r \in \mathcal{S}_r}\nabla \Fr(\yr) - \nabla \Fr(\phir)\|^2 + \frac{\sigma^2}{KS} \\
    &\leq 2 \beta \E_{\mathcal{S}_r} [\frac{1}{S} \sum_{i_r \in \mathcal{S}_r} \Fr(\phir) - \Fr(\yr) - \langle \nabla \Fr(\yr), \phir - \yr \rangle] + \frac{\sigma^2}{KS} \\
    &= 2 \beta [\frac{1}{N}\sum_{i=1}^N \tilde{F}_i(\phi_i^{(r)}) - \tilde{F}_i(y_i^{(r)}) - \frac{1}{N} \sum_{i=1}^N \langle \nabla \tilde{F}_i(y_i^{(r)}), \phi_i^{(r)} - y_i^{(r)}\rangle] + \frac{\sigma^2}{KS}
\end{align}

From convexity we have that
\begin{align}
    &\Fr(\yr) - \Fr(x^*) \\
    &\leq \langle \nabla \Fr(\yr), \yr - x^* \rangle \\ 
    &= \frac{1 - \tau}{\tau} \langle \nabla \Fr(\yr), \phir - \yr \rangle + \langle \nabla \Fr(\yr), x^{(r)} - x^* \rangle \\
    &= \frac{1 - \tau}{\tau} \langle \nabla \Fr(\yr), \phir - \yr \rangle + \langle \nabla \Fr(\yr) - \gr, x^{(r)} - x^* \rangle + \langle \gr, x^{(r)} - x^{(r+1)}\rangle + \langle \gr, x^{(r+1)} - x^* \rangle
\end{align}
where the second to last inequality comes from the definition that $\yr = \tau x^{(r)} + (1 - \tau) \phir$.
Taking expectation with respect to the sampled clients, we have
\begin{align}
    \label{eq:mirror-acc}
    \frac{1}{N} \sum_{i=1}^N \tilde{F}_i(y_i^{(r)}) - \tilde{F}(x^*) \leq \frac{1 - \tau}{\tau N} \sum_{i=1}^N \langle \nabla \tilde{F}_i(y_i^{(r)}), \phi_i^{(r)} - y_i^{(r)} \rangle + \E_{\mathcal{S}_r} \langle \gr, x^{(r)} - x^{(r+1)} \rangle + \E_{\mathcal{S}_r} \langle \gr, x^{(r+1)} - x^* \rangle
\end{align}
For $\E_{\mathcal{S}_r} \langle \gr, x^{(r)} - x^{(r+1)} \rangle$, we can employ smoothness at $(\phi_{I_r}^{(r+1)}, y_{I_r}^{(r)})$, which holds for any $I_r \in \mathcal{S}_r'$:
\begin{align}
    \tilde{F}_{I_r}(\phi_{I_r}^{(r+1)}) - \tilde{F}_{I_r}(y_{I_r}^{(r)}) \leq \langle \nabla \tilde{F}_{I_r}(y_{I_r}^{(r)}),  \phi_{I_r}^{(r+1)} - y_{I_r}^{(r)} \rangle + \frac{\beta}{2} \|\phi_{I_r}^{(r+1)} - y_{I_r}^{(r)}\|^2
\end{align}
using $\phi^{(r+1)}_{I_r} = \tau x^{(r + 1)} + (1 - \tau)\phi^{(r)}_{I_r}$ and $y_{I_r}^{(r)} = \tau x^{(r)} + (1 - \tau) \phi_{I_r}^{(r)}$ (though the second is never explicitly computed and only implicitly exists)
\begin{align}
    \tilde{F}_{I_r}(\phi_{I_r}^{(r+1)}) - \tilde{F}_{I_r}(y_{I_r}^{(r)}) \leq \tau \langle \nabla \tilde{F}_{I_r}(y_{I_r}^{(r)}),  x^{(r+1)} - x^{(r)} \rangle + \frac{\beta \tau^2}{2} \|x^{(r+1)} - x^{(r)}\|^2
\end{align}

Taking expectation over $\mathcal{S}_r'$ and using $\phi^{(r+1)}_{I_r} = \tau x^{(r + 1)} + (1 - \tau)\phi^{(r)}_{I_r}$ and $y_{I_r}^{(r)} = \tau x^{(r)} + (1 - \tau) \phi_{I_r}^{(r)}$  we see that 
\begin{align}
    \E_{\mathcal{S}_r'}[\frac{1}{S} \sum_{I_r \in \mathcal{S}_r'} \tilde{F}_{I_r}(\phi_{I_r}^{(r+1)})] - \frac{1}{N} \sum_{i=1}^N \tilde{F}_i(y_i^{(r)}) \leq \tau \langle \frac{1}{N} \sum_{i=1}^N\nabla \tilde{F}_i(y_i^{(r)}), x^{(r+1)} - x^{(r)} \rangle + \frac{\beta \tau^2}{2} \|x^{(r+1)} - x^{(r)} \|^2
\end{align}
and rearranging, 
\begin{align}
    &\langle \gr, x^{(r)} - x^{(r+1)} \rangle \\
    &\leq \frac{1}{\tau N} \sum_{i=1}^N \tilde{F}_i(y_i^{(r)}) - \frac{1}{\tau S} \E_{\mathcal{S}_r'}[ \sum_{I_r \in \mathcal{S}_r'} \tilde{F}_{I_r}(\phi_{I_r}^{(r+1)})] + \langle \frac{1}{N} \sum_{i=1}^N \nabla \tilde{F}_i(y_i^{(r)}) - \gr, x^{(r+1)} - x^{(r)} \rangle + \frac{\beta \tau}{2} \|x^{(r+1)} - x^{(r)} \|^2
\end{align}
Substituting this into \cref{eq:mirror-acc} after taking expectation over $\mathcal{S}_r$, and observing that from \citep{zhou2019direct}
\begin{align}
    \langle \gr, x^{(r + 1)} - u \rangle \leq - \frac{1}{2 \eta} \|x^{(r + 1)} - x^{(r)}\|^2 + \frac{1}{2 \eta} \|x^{(r)} - u\|^2 - \frac{1 + \eta \mu}{2 \eta} \|x^{(r + 1)} - u\|^2 + h(u) - h(x^{(r + 1)})
\end{align}
so with $u = x^*$, we get
\begin{align}
    &\frac{1}{N} \sum_{i=1}^N \tilde{F}_i(y_i^{(r)}) - \tilde{F}(x^*) \\
    &\leq \frac{1 - \tau}{\tau N} \sum_{i=1}^N \langle \nabla \tilde{F}_i(y_i^{(r)}), \phi_i^{(r)} - y_i^{(r)} \rangle + \frac{1}{\tau N} \sum_{i=1}^N \tilde{F}_i(y_i^{(r)}) - \frac{1}{\tau S} \E_{\mathcal{S}_r, \mathcal{S}_r'}[ \sum_{I_r \in \mathcal{S}_r'} \tilde{F}_{I_r}(\phi_{I_r}^{(r+1)})] \\
    & \ \ \ + \E_{\mathcal{S}_r }\langle \frac{1}{N} \sum_{i=1}^N \nabla \tilde{F}_i(y_i^{(r)}) - \gr, x^{(r+1)} - x^{(r)} \rangle + \frac{\beta \tau}{2} \E_{\mathcal{S}_r } \|x^{(r+1)} - x^{(r)} \|^2  \\
    & \ \ \ - \frac{1}{2 \eta} \E_{\mathcal{S}_r} \|x^{(r + 1)} - x^{(r)}\|^2 + \frac{1}{2 \eta} \|x^{(r)} - x^*\|^2 - \frac{1 + \eta \mu}{2 \eta} \E_{\mathcal{S}_r} \|x^{(r + 1)} - x^*\|^2 + h(x^*) - \E_{\mathcal{S}_r} h(x^{(r + 1)})
\end{align}
We use the constraint that $\beta \tau \leq \frac{1}{\eta} - \frac{\beta \tau}{1 - \tau}$ plus Young's inequality $\langle a, b \rangle \leq \frac{1}{2 c} \|a\|^2 + \frac{c}{2} \|b\|^2$ with $c = \frac{\beta \tau}{1 - \tau}$ on $\E_{\mathcal{S}_r }\langle \frac{1}{N} \sum_{i=1}^N \nabla \tilde{F}_i(y_i^{(r)}) - \gr, x^{(r+1)} - x^{(r)} \rangle$ to get 
\begin{align}
    &\frac{1}{N} \sum_{i=1}^N \tilde{F}_i(y_i^{(r)}) - \tilde{F}(x^*) \\
    &\leq \frac{1 - \tau}{\tau N} \sum_{i=1}^N \langle \nabla \tilde{F}_i(y_i^{(r)}), \phi_i^{(r)} - y_i^{(r)} \rangle + \frac{1}{\tau N} \sum_{i=1}^N \tilde{F}_i(y_i^{(r)}) - \frac{1}{\tau S} \E_{\mathcal{S}_r, \mathcal{S}_r'}[ \sum_{I_r \in \mathcal{S}_r'} \tilde{F}_{I_r}(\phi_{I_r}^{(r+1)})] \\
    & \ \ \ + \frac{1 - \tau}{2 \beta \tau} \E_{\mathcal{S}_r }\| \frac{1}{N} \sum_{i=1}^N \nabla \tilde{F}_i(y_i^{(r)}) - \gr\|^2  + \frac{1}{2 \eta} \|x^{(r)} - x^*\|^2 - \frac{1 + \eta \mu}{2 \eta} \E_{\mathcal{S}_r} \|x^{(r + 1)} - x^*\|^2 + h(x^*) - \E_{\mathcal{S}_r} h(x^{(r + 1)})
\end{align}
using the bound on variance, we get 
\begin{align}
    &\frac{1}{N} \sum_{i=1}^N \tilde{F}_i(y_i^{(r)}) - \tilde{F}(x^*) \\
    &\leq  \frac{1}{\tau N} \sum_{i=1}^N \tilde{F}_i(y_i^{(r)}) - \frac{1}{\tau S} \E_{\mathcal{S}_r, \mathcal{S}_r'}[ \sum_{I_r \in \mathcal{S}_r'} \tilde{F}_{I_r}(\phi_{I_r}^{(r+1)})] + \frac{1 - \tau}{\tau N} \sum_{i=1}^N \tilde{F}_i(\phi_i^{(r)}) - \tilde{F}_i(y_i^{(r)})\\
    & \ \ \  + \frac{1}{2 \eta} \|x^{(r)} - x^*\|^2 - \frac{1 + \eta \mu}{2 \eta} \E_{\mathcal{S}_r} \|x^{(r + 1)} - x^*\|^2 + h(x^*) - \E_{\mathcal{S}_r} h(x^{(r + 1)}) + \frac{(1 - \tau)\sigma^2}{2 \beta \tau KS}
\end{align}
combining terms,
\begin{align}
    &\frac{1}{\tau S} \E_{\mathcal{S}_r, \mathcal{S}_r'}[ \sum_{I_r \in \mathcal{S}_r'} \tilde{F}_{I_r}(\phi_{I_r}^{(r+1)})] - F(x^*) \\
    &\leq  \frac{1 - \tau}{\tau N} \sum_{i=1}^N \tilde{F}_i(\phi_i^{(r)}) + \frac{1}{2 \eta} \|x^{(r)} - x^*\|^2 - \frac{1 + \eta \mu}{2 \eta} \E_{\mathcal{S}_r} \|x^{(r + 1)} - x^*\|^2 - \E_{\mathcal{S}_r} h(x^{(r + 1)}) + \frac{(1 - \tau)\sigma^2}{2 \beta \tau KS}
\end{align}
Using convexity of $h$ and $\phi_{I_k}^{(r+1)} = \tau x^{(r+1)} + (1 - \tau) \phi_{I_k}^{(r)}$ for $I_k \in \mathcal{S}_r'$,
\begin{align}
    h(\phi_{I_k}^{(r+1)}) \leq \tau h(x^{(r+1)}) + (1 - \tau) h(\phi_{I_k}^{(r)})
\end{align}
After taking expectation with respect to $\mathcal{S}_r$ and $\mathcal{S}_r'$,
\begin{align}
    -\E_{\mathcal{S}_r}[h(x^{(r+1)})] \leq \frac{1 - \tau}{\tau N} \sum_{i=1}^N h(\phi_i^{(r)}) - \frac{1}{\tau} \E_{\mathcal{S}_r, \mathcal{S}_r'}[\frac{1}{S} \sum_{I_r \in \mathcal{S}_r'} h(\phi_{I_k}^{(r+1)})]
\end{align}
and plugging this back in, multiplying by $S/N$ on both sides, and adding both sides by $\frac{1}{\tau N} \E_{\mathcal{S}_r'} [\sum_{i \notin \mathcal{S}_r'} (F_i(\phi_i^{(r)}) - F_i(x^*))]$
\begin{align}
    \frac{1}{\tau } \E_{\mathcal{S}_r, \mathcal{S}_r'}[ \frac{1}{N} \sum_{i=1}^N  F_{i}(\phi_{i}^{(r+1)}) - F_{i}(x^*)] 
    &\leq  \frac{(1 - \tau)S}{\tau N} (\frac{1}{N} \sum_{i=1}^N F_i(\phi_i^{(r)}) - F_i(x^*)) + \frac{1}{\tau N} \E_{\mathcal{S}_r'} [\sum_{i \notin \mathcal{S}_r'} (F_i(\phi_i^{(r)}) - F_i(x^*))] \\
    & \ \ \ + \frac{S}{2 \eta N} \|x^{(r)} - x^*\|^2 - \frac{(1 + \eta \mu)S}{2 \eta N} \E_{\mathcal{S}_r} \|x^{(r + 1)} - x^*\|^2 + \frac{(1 - \tau)\sigma^2}{2 \beta \tau KN}
\end{align}
Observe that the probability of choosing any client index happens with probability $S/N$, so
\begin{align}
    \frac{1}{\tau N} \E_{\mathcal{S}_r'} [\sum_{i \notin \mathcal{S}_r'} (F_i(\phi_i^{(r)}) - F_i(x^*))] = \frac{N - S}{\tau N} (\frac{1}{N} \sum_{i=1}^N F_i(\phi_i^{(r)}) - F_i(x^*))
\end{align}
which implies 
\begin{align}
    \frac{1}{\tau } \E_{\mathcal{S}_r, \mathcal{S}_r'}[ \frac{1}{N} \sum_{i=1}^N  F_{i}(\phi_{i}^{(r+1)}) - F_{i}(x^*)] 
    &\leq  \frac{1 - \frac{\tau S}{N}}{\tau } (\frac{1}{N} \sum_{i=1}^N F_i(\phi_i^{(r)}) - F_i(x^*)) \\
    & \ \ \ + \frac{S}{2 \eta N} \|x^{(r)} - x^*\|^2 - \frac{(1 + \eta \mu)S}{2 \eta N} \E_{\mathcal{S}_r} \|x^{(r + 1)} - x^*\|^2 + \frac{(1 - \tau)\sigma^2}{2 \beta \tau KN}
\end{align}
To complete our Lyapunov function, we need another term:
\begin{align}
    -\frac{1}{N} \sum_{i=1}^N \langle \nabla F_i(x^*), \phi_i^{(r+1)} - x^* \rangle &= -\frac{1}{N} \sum_{I_r \in \mathcal{S}_r'} \langle \nabla F_{I_r}(x^*), \phi^{(r+1)}_{I_r} - x^* \rangle - \frac{1}{N} \sum_{j \notin \mathcal{S}_r'} \langle \nabla F_j(x^*), \phi^{(r)}_{j} - x^* \rangle \\
    &= \sum_{I_r \in \mathcal{S}_r'} -\frac{\tau}{N} \langle \nabla F_{I_r}(x^*), x^{(r+1)} - x^* \rangle + \frac{\tau}{N} \langle \nabla F_{I_r}(x^*), \phi_{I_r}^{(r)} - x^* \rangle \\
    & \ \ \ - \frac{1}{N} \sum_{i=1}^N \langle \nabla F_i(x^*), \phi_i^{(r)} - x^* \rangle
\end{align}
Taking expectation with respect to $\mathcal{S}_r, \mathcal{S}_r'$,
\begin{align}
    \E_{\mathcal{S}_r, \mathcal{S}_r'} [-\frac{1}{N} \sum_{i=1}^N \langle \nabla F_i(x^*), \phi_i^{(r+1)} - x^* \rangle] = -(1 - \frac{\tau S}{N})(\frac{1}{N} \sum_{i=1}^N \langle \nabla F_i(x^*), \phi_i^{(r)} - x^* \rangle)
\end{align}
Let $B_r := \frac{1}{N} \sum_{i=1}^N F_i(\phi_i^{(r)}) - F(x^*) - \frac{1}{N} \sum_{i=1}^N \langle \nabla F_i(x^*), \phi_i^{(r)} - x^* \rangle$ and $P_r := \|x^{(r)} - x^* \|^2$, then we can write 
\begin{align}
    \frac{1}{\tau} \E_{\mathcal{S}_r, \mathcal{S}_r'}[B_{r+1}] + \frac{(1 + \eta \mu) S}{2 \eta N} \E_{\mathcal{S}_r} [P_{r+1}] \leq \frac{1 - \frac{\tau S}{N}}{\tau} B_r + \frac{S}{2 \eta N} P_r + \frac{(1 - \tau)\sigma^2}{2 \beta \tau KN} 
\end{align}

\textbf{Case 1:} Suppose that $\frac{(N/S)}{\kappa } \leq \frac{3}{4}$, then choosing $\eta = \sqrt{\frac{1}{3 \mu (N/S) \beta}}$, $\tau = \frac{(N/S) \eta \mu}{1 + \eta \mu} = \frac{\sqrt{\frac{(N/S)}{3 \kappa}}}{1 + \sqrt{\frac{1}{3 (N/S) \kappa}}} < \frac{1}{2}$, we evaluate the parameter constraint $\beta \tau \leq \frac{1}{\eta} - \frac{\beta \tau}{1 - \tau}$:
\begin{align}
    \beta \tau \leq \frac{1}{\eta} - \frac{\beta \tau}{1 - \tau} \implies (1 + \frac{1}{1 - \tau}) \tau \leq \frac{1}{\beta \eta} \implies \frac{2 - \tau}{1 - \tau} \frac{\sqrt{\frac{(N/S)}{3 \kappa}}}{1 + \sqrt{\frac{1}{3 (N/S) \kappa}}} \leq \sqrt{\frac{3(N/S)}{\kappa}}
\end{align}
which shows our constraint is satisfied.  We also know that 
\begin{align}
    \frac{1}{\tau(1 + \eta \mu)} = \frac{1 - \frac{\tau S}{N}}{\tau}=\frac{1}{(N/S) \eta \mu} 
\end{align}
So we can write
\begin{align}
    \frac{1}{(N/S) \eta \mu} \E_{\mathcal{S}_r, \mathcal{S}_r'}[B_{r+1}] + \frac{1}{2 \eta (N/S)} \E_{\mathcal{S}_r}[P_{r+1}] \leq (1 + \eta \mu)^{-1} (\frac{1}{(N/S) \eta \mu} B_r + \frac{1}{2 \eta (N/S)} P_r) + \frac{(1 - \tau)\sigma^2}{2 \beta \tau KN} 
\end{align}
Telescoping the contraction and taking expectation with respect to all randomness, we have 
\begin{align}
    \frac{1}{(N/S) \eta \mu} \E[B_{R}] + \frac{1}{2 \eta (N/S)} \E[P_{R}] \leq (1 + \eta \mu)^{-R} (\frac{1}{(N/S) \eta \mu} \E B_0 + \frac{1}{2 \eta (N/S)} \E P_0) + \frac{(1 - \tau)\sigma^2}{2 \beta \tau KN} (\frac{1 + \eta \mu}{\eta \mu})
\end{align}
$B_0 = F(x^{(0)}) - F(x^*)$ and $\E B_R \geq 0$ based on convexity.  Substituting the parameter choices,
\begin{align}
    \E\|x^{(R)} - x^*\|^2 \leq (1 + \sqrt{\frac{1}{3(N/S) \kappa}})^{-R} (\frac{2}{\mu} \Delta + D^2) + \frac{4 \sqrt{\kappa} \sigma^2}{\beta \mu K S}
\end{align}

\textbf{Case 2:} On the other hand, we can have $\frac{(N/S)}{\kappa} > \frac{3}{4}$ and choose $\eta = \frac{1}{2\mu (N/S)}$, $\tau = \frac{(N/S) \eta \mu}{1 + \eta \mu} = \frac{(1/2)}{1 + \frac{1}{2 (N/S)}} < \frac{1}{2}$.  One can check that the constraint $\beta \tau \leq \frac{1}{\eta} - \frac{\beta \tau}{1 - \tau}$ is satisfied.  

After telescoping and taking expectation,
\begin{align}
    2\E[B_{R}] + \frac{1}{2 \eta (N/S)} \E[P_{R}] \leq (1 + \eta \mu)^{-R} (2 \E B_0 + \frac{1}{2 \eta (N/S)} \E P_0) + \frac{(1 - \tau)\sigma^2}{2 \beta \tau KN} (\frac{1 + \eta \mu}{\eta \mu})
\end{align}
which gives us
\begin{align}
    \E \|x^{(R)} - x^*\|^2 \leq (1 + \frac{1}{2 (N/S)})^{-R}(\frac{2}{\mu} \Delta + D^2) + \frac{4 \sigma^2}{\beta \mu K S}
\end{align}
Altogether, supposing we choose our parameters as stated in the two cases, we have:
\begin{align}
    \E F(x^{(R)}) - F(x^*) \leq \mathcal{O}(\kappa \Delta \exp(-\min\{\frac{S}{N}, \sqrt{\frac{S}{N \kappa}}\}R) + \frac{\sqrt{\kappa} \sigma^2}{\mu K S})
\end{align}
\subsection{\mbsgd}
\begin{proposition}
    \label{thm:strongsgd}
    Given $\mu$-strong convexity \pcref{asm:strongconvex}, $\beta$-smoothness of $F$ \pcref{asm:smooth}, and $\sigma^2$ variance of $g_{i,k}^{(r)}$'s \pcref{asm:uniform_variance}, then SGD \pcref{algo:mbsgd} with
    \begin{align}
        \eta = \min \{ \frac{1}{\beta}, \frac{\log(\max\{e, \frac{2 \mu^2 \Delta NKR}{\beta \sigma^2}\})}{\mu R} \}
    \end{align}
    and defining
    \begin{align}
        \Phi := \log(\max\{e, \frac{2 \mu^2 \Delta NKR}{\beta \sigma^2}\})
    \end{align}
    Achieves convergence rate
    \begin{align}
        \E F(x^{(R)}) - F(x^*) \leq \Delta \exp(-\frac{R}{\kappa}) + \frac{\beta \sigma^2}{\mu^2 N K R} \Phi
    \end{align}
\end{proposition}
\begin{proof}
    By \cref{lemma:strongpl}, $\mu$-strong convexity implies $\mu$-PL.  Therefore, by \cref{thm:plsgd}, the theorem statement holds.
\end{proof}
\subsection{\asg}
\begin{proposition}
    \label{thm:appasg}
    Consider ASG \pcref{algo:ambsgd}.  Given $\beta$-smoothness of $F_i$'s \pcref{asm:smooth}, $\mu$-strong convexity of $F_i$'s \pcref{asm:strongconvex}, and a uniform upper bound on client gradient variance \pcref{asm:uniform_variance}, if we set
    \begin{align}
        \eta = \min\{\frac{1}{\beta}, \frac{\log(\max\{e, \min \{\frac{2 \Delta  \mu N K R}{\sigma^2}, \frac{2 \Delta \mu^2  N K R^3  }{\beta \sigma^2}\}\})}{\mu R^2 } \}
    \end{align} 
	\begin{align}
		\text{let } \Phi = \log(\max\{e, \min \{\frac{2 \Delta  \mu N K R}{\sigma^2}, \frac{2 \Delta \mu^2  N K R^3  }{\beta \sigma^2}\}\}) \text{  ,   then}
	\end{align}
    \begin{align}
        \E F(x^{(R + 1)}) - F(x^*) \leq 2 \Delta \exp(- \frac{R}{\sqrt{\kappa}}) +  \frac{\sigma^2}{\mu N K R} \Phi^{1/2} + \frac{\beta \sigma^2}{\mu^2 N K R^3} \Phi^{3/2}
    \end{align}
\end{proposition}
\begin{proof}
    From \citep{aybat2019universally} (Eq.13), we know that
    \begin{align}
        \E V_{r + 1} \leq (1 - \sqrt{\eta \mu})( \E V_{r}) + \frac{\sigma^2 \eta}{2 NK}(1 + \eta \beta)
    \end{align}
    where $V_r$ is such that $F(x^{(r)}) - F(x^*) \leq V_r \leq 2(F(x^{(r)}) - F(x^*))$.

If we unroll this, we get 
\begin{align}
    \E V_{R + 1} &\leq (1 - \sqrt{\eta \mu})^R \E V_1 + \frac{\sigma^2 \eta^{1/2}}{2 \mu^{1/2} NK} + \frac{\sigma^2 \eta^{3/2} \beta}{2 \mu^{1/2}NK} \\
    &\leq \exp( - \sqrt{\eta\mu} R)\E V_1 + \frac{\sigma^2 \eta^{1/2}}{2 \mu^{1/2}NK} + \frac{\sigma^2 \eta^{3/2} \beta}{2 \mu^{1/2}NK} 
\end{align}
Now if 
\begin{align}
    \eta = \min\{\frac{1}{\beta}, \frac{\log(\max\{e, \min \{\frac{2 \Delta  \mu N K R}{\sigma^2}, \frac{2 \Delta \mu^2  N K R^3  }{\beta \sigma^2}\}\})}{\mu R^2 } \}
\end{align} 

So altogether, we have that 
\begin{align}
    \E F(x^{(R + 1)}) - F(x^*) \leq 2 \Delta \exp(- \frac{R}{\sqrt{\kappa}}) +  \frac{\sigma^2}{\mu N K R} \Phi^{1/2} + \frac{\beta \sigma^2}{\mu^2 N K R^3} \Phi^{3/2}
\end{align}
where 
\begin{align}
    \Phi = \log(\max\{e, \min \{\frac{2 \Delta  \mu N K R}{\sigma^2}, \frac{2 \Delta \mu^2  N K R^3  }{\beta \sigma^2}\}\})
\end{align}
\end{proof}
\subsection{\lsgd}
\begin{theorem}
    \label{thm:fedavgstrong}
    Suppose we run \Lsgd \pcref{algo:fedavg} with a few modifications:
    \begin{enumerate}
        \item Each client performs $\sqrt{K}$ local steps per round
        \item Each local step is computed as $g_{i,k}^{(r)} = \frac{1}{\sqrt{K}} \sum_{b=0}^{\sqrt{K} - 1} \nabla f(x_{i,k}^{(r)}; z_{i,k\sqrt{K} + b}^{(r)})$ where $z_{i,j}^{(r)} \sim \mathcal{D}_i$
    \end{enumerate}
    Then given $\mu$-strong convexity \pcref{asm:pl} of $F_i$, $\beta$-smoothness of $F_i$'s \pcref{asm:smooth}, $\zeta^2$-heterogeneity of $F_i$'s \pcref{asm:grad_het}, upper bound on initial function suboptimality \pcref{asm:subopt}, and a uniform upper bound of variance $\sigma^2$ \pcref{asm:uniform_variance}, if we choose 
    \begin{align}
        \eta = \frac{1}{2\beta}
    \end{align}
    then
    \begin{align}
        \E F(x^{(R)}) - F(x^*) \leq \Delta \exp(-\frac{R\sqrt{K}}{\kappa}) + \frac{\zeta^2}{2 \mu} + \frac{\sigma^2}{2\mu \sqrt{K}}
    \end{align}
    where $K$ is a square number. \footnote{That $K$ is square is assumed for technical simplicity--the proof can be easily generalized.}

    Next, if we are in the setting where $\sigma^2 = 0$, then we have for every iterate in the algorithm's execution:
    \begin{align}
        \|x_{i,k}^{(r)} - x^*\|^2 \leq \tilde{\mathcal{O}}(D^2 + \frac{\zeta^2}{\mu^2})
    \end{align}
\end{theorem}
\begin{proof}
    By smoothness of F \pcref{asm:smooth}, we have for $k \in \{0, \dots, \sqrt{K} - 1\}$
    \begin{align}
        F(x^{(r)}_{i, k+1}) - F(x^{(r)}_{i, k}) \leq - \eta \langle \nabla F(x^{(r)}_{i, k}),  g_{i,k}^{(r)} \rangle + \frac{\beta \eta^2}{2} \|g_{i,k}^{(r)}\|^2
    \end{align}
    Using the fact that for any $a,b$ we have $-2ab = (a-b)^2 - a^2 - b^2$,
    \begin{align}
        F(x^{(r)}_{i, k+1}) - F(x^{(r)}_{i, k}) \leq - \frac{\eta}{2} \|\nabla F(x^{(r)}_{i, k})\|^2 + \frac{\beta \eta^2 - \eta}{2}\| g_{i,k}^{(r)}\|^2 + \frac{\eta}{2} \| g_{i,k}^{(r)} - \nabla F(x^{(r)}_{i, k})\|^2
    \end{align}
    Letting $\eta \leq \frac{1}{\beta}$,
    \begin{align}
        F(x^{(r)}_{k+1}) - F(x^{(r)}_{i,k}) \leq - \frac{\eta}{2} \|\nabla F(x^{(r)}_{i,k})\|^2 + \frac{\eta}{2} \| g_{i,k}^{(r)} - \nabla F(x^{(r)}_{i,k})\|^2
    \end{align}
    Conditioning on everything up to the $k$-th step of the $r$-th round,
    \begin{align}
        \E_{r,k} F(x^{(r)}_{i, k+1}) - F(x^{(r)}_{i,k}) &\leq - \frac{\eta}{2} \|\nabla F(x^{(r)}_{i,k})\|^2 + \frac{\eta}{2} \E_{r,k} \| g_{i,k}^{(r)} - \nabla F(x^{(r)}_{i,k})\|^2 \\
        &\leq - \frac{\eta}{2} \|\nabla F(x^{(r)}_{i,k})\|^2 + \frac{\eta \zeta^2}{2}   + \frac{\eta \sigma^2}{2 \sqrt{K}}
    \end{align}
    Where the last step used the fact that $\E[X^2] = \text{Var}(X) + \E[X]$, the assumption on heterogeneity \pcref{asm:grad_het}, and the assumption on gradient variance \pcref{asm:uniform_variance} along with the fact that $g_{i,k}^{(r)}$ is an average over $\sqrt{K}$ client gradient queries.
    Next, using $\mu$-strong convexity of $F$ \pcref{asm:strongconvex} along with \cref{lemma:strongpl},
    \begin{align}
        \E_{r,k} F(x^{(r)}_{i, k+1}) - F(x^{(r)}_{i,k}) \leq - \eta \mu (F(x^{(r)}_{i,k}) - F(x^*)) + \frac{\eta \zeta^2}{2}   + \frac{\eta \sigma^2}{2 \sqrt{K}}
    \end{align}
    which after taking full expectation gives
    \begin{align}
        \E F(x^{(r)}_{i, k+1}) - F(x^*) \leq (1 - \eta \mu)(\E F(x^{(r)}_{i, k}) - F(x^*)) + \frac{\eta \zeta^2}{2} + \frac{\eta \sigma^2}{2 \sqrt{K}}
    \end{align}
    Unrolling the recursion over $k$ we get 
    \begin{align}
        \E F(x^{(r)}_{i, K}) - F(x^*) \leq (1 - \eta \mu)^{\sqrt{K}} (\E F(x^{(r)}_{i,0}) - F(x^*)) + (\frac{\eta \zeta^2}{2 } + \frac{\eta \sigma^2}{2 \sqrt{K}}) \sum_{k=0}^{\sqrt{K}-1} (1 - \eta \mu)^k
    \end{align}
    Also note that $x^{(r + 1)} = \frac{1}{S} \sum_{i \in \mathcal{S}_r} x^{(r)}_{i, K}$.  So by convexity of $F$,
    \begin{align}
        \E F(x^{(r + 1)}) - F(x^*) &\leq \frac{1}{S} \sum_{i \in \mathcal{S}_r} \E F(x^{(r)}_{i, K}) - F(x^*)\\
        &\leq (1 - \eta \mu)^{\sqrt{K}} (\E F(x^{(r)}) - F(x^*)) + (\frac{\eta \zeta^2}{2 } + \frac{\eta \sigma^2}{2 \sqrt{K}}) \sum_{k=0}^{\sqrt{K}-1} (1 - \eta \mu)^k
    \end{align}
    Unrolling the recursion over $R$, we get
    \begin{align}
        \E F(x^{(R)}) - F(x^*) \leq (1 - \eta \mu)^{R\sqrt{K}} (F(x^{(0)}) - F(x^*)) + (\frac{\eta \zeta^2}{2 } + \frac{\eta \sigma^2}{2 \sqrt{K}}) \sum_{r=0}^{R-1} \sum_{k=0}^{\sqrt{K}-1} (1 - \eta \mu)^{r\sqrt{K} + k}
    \end{align}
    Which can be upper bounded as 
    \begin{align}
        \E F(x^{(R)}) - F(x^*) \leq (1 - \eta \mu)^{R\sqrt{K}} (F(x^{(0)}) - F(x^*)) + \frac{\zeta^2}{2 \mu} + \frac{\sigma^2}{2\mu\sqrt{K}}
    \end{align}

    Next we prove the distance bound under zero noise.  Take $K$ steps per round and batches of size 1.  For some client $i$ on round $r$, we shorthand $x_{i,k}^{(r)}$ as $x_k$
    \begin{align}
        \|x_k - x^*\|^2 &= \|x_{k-1} - \eta \nabla F_i(x_k) - x^*\|^2 \\
        &= \|x_{k-1} - x^*\|^2 - 2 \eta \langle \nabla F_i(x_k), x_k - x^* \rangle + \eta^2 \|\nabla F_i(x_k)\|^2 
    \end{align}
    We start by bounding the middle term.
    \begin{align}
        - 2 \eta \langle \nabla F_i(x_k), x_k - x^* \rangle  &= -2 \eta(\langle \nabla  F(x_k), x_k - x^* \rangle + \langle \nabla  F_i(x_k) - F(x_k), x_k - x^* \rangle)
    \end{align}
    The first term can be upper bounded using strong convexity \cref{asm:strongconvex}:
    \begin{align}
        -\langle \nabla  F(x_k), x_k - x^* \rangle \leq -(F(x_k) - F(x^*) + \frac{\mu}{2}\|x_k - x^*\|^2)
    \end{align}
    The second term can be upper bounded using the Fenchel-Young inequality:
    \begin{align}
        -\langle \nabla  F_i(x_k) - F(x_k), x_k - x^* \rangle &\leq \frac{1}{ \mu} \|\nabla F_i(x_k) - \nabla F(x_k)\|^2 + \frac{\mu}{4} \|x_k - x^*\|^2 \\
        &\leq \frac{\zeta^2}{ \mu}  + \frac{\mu}{4} \|x_k - x^*\|^2
    \end{align}
    Next, we upper bound the third term.
    \begin{align}
        \eta^2\|\nabla F_i(x_k)\|^2 &= 2 \eta^2\|\nabla F_i(x_k) - \nabla F(x_k)\|^2 + 2\eta^2\|\nabla F(x_k) - \nabla F(x^*)\|^2 \\
        &\leq 2 \eta^2 \zeta^2 + 4 \beta \eta^2 (F(x_k) - F(x^*))
    \end{align}
    where in the last step we used smoothness \cref{asm:smooth} for the first term and the definition of $\hat{\zeta}_*^2$ for the second term.

    We can substitute all our upper bounds to get

    \begin{align}
        & \|x_k - x^*\|^2 \\
        &\leq (1 - \eta \mu + \frac{\eta \mu}{2} )\|x_{k-1} - x^*\|^2 - 2\eta(2 \beta \eta - 1)(F(x_k) - F(x^*)) + \frac{2 \eta_1 \zeta^2}{\mu} + 2 \eta^2 \zeta^2
    \end{align}
    Setting $\eta \leq \frac{1}{2 \beta}$, we have
    \begin{align}
        \|x_k - x^*\|^2 \leq (1 - \frac{\eta_1 \mu}{4})\|x_{k-1} - x^*\|^2 + \frac{3 \eta \zeta^2}{\mu} 
    \end{align}
    Unrolling,
    \begin{align}
        \|x_K - x^*\|^2 \leq (1 - \frac{\eta_1 \mu}{4})^K \|x_{0} - x^*\|^2 + \frac{3 \eta \zeta^2}{\mu} \sum_{k=0}^{K-1} (1 - \frac{\eta \mu}{4})^k
    \end{align}
    Now recall that $x^{(r + 1)} = \frac{1}{S} \sum_{i \in \mathcal{S}_r} x_{i,K}^{(r)}$.  So by convexity of the distance function,
    \begin{align}
        \|x^{(r+1)} - x^*\|^2 \leq \frac{1}{S} \sum_{i \in \mathcal{S}_r} x_{i,K}^{(r)} \|x_{i,K}^{(r)} - x^*\|^2 \leq (1 - \frac{\eta \mu}{4})^K \|x^{(r)} - x^*\|^2 + \frac{3 \eta \zeta^2}{\mu} \sum_{k=0}^{K-1} (1 - \frac{\eta \mu}{4})^k
    \end{align}
    Further unrolling,
    \begin{align}
        \|x^{(R)} - x^*\|^2 &\leq (1 - \frac{\eta \mu}{4})^{RK} \|x^{(0)} - x^*\|^2 + \frac{3 \eta \zeta^2}{\mu} \sum_{r=0}^{R-1} \sum_{k=0}^{K-1} (1 - \frac{\eta \mu}{4})^{rK + k} \\
        &\leq (1 - \frac{\eta \mu}{4})^{RK} \|x^{(0)} - x^*\|^2 + \frac{12 \zeta^2}{\mu^2}
    \end{align}
\end{proof}
\subsection{M-\lsgd}
\begin{proposition}
    \label{thm:mfedavg}
    Assume that $F_i$'s are $\beta$-smooth \pcref{asm:smooth}, $\zeta^2$-heterogeneous \pcref{asm:grad_het}, have $\sigma^2$ gradient variance on client gradient queries \pcref{asm:uniform_variance}.  
    
    Run M-\lsgd \pcref{algo:m-lsgd} with the settings $\eta_{s + 1} = \eta/2^{s}$ and $R_s = \frac{2^{s} \log(4)}{\mu \eta K}$ for $s \geq 2$.  Let $R = \sum_{s=1}^S R_s$.  

    Then if we let  
    \begin{align}
        \eta = \min \{ \frac{1}{10 \beta}, \frac{\log(\max \{e, \min \{\frac{\mu^2 D^2 N K R_1}{3 \sigma^2}, \frac{\mu^3 D^2 K^2 R_1^2}{6 \beta  (\sigma^2 + 2 K \zeta^2)})}{\mu K R_1} \}
    \end{align}
    and let 
    \begin{align}
        \Phi = \log(\max \{e, \min \{\frac{\mu^2 D^2 N K R_1}{3 \sigma^2}, \frac{\mu^3 D^2 K^2 R_1^2}{6 \beta  (\sigma^2 + 2 K \zeta^2)})
    \end{align}
    we have the following convergence rate:

    \begin{align}
        F(x^{(s, R_s)}) - F(x^*) \leq \frac{1}{2^{S-1}}(\beta D^2 \exp(-\frac{R_1 K}{10 \kappa}) + \frac{6 \beta \sigma^2}{\mu^2 N K R_1} \Phi + \frac{12 \beta^2 \sigma^2}{\mu ^3 K R_1^2} \Phi^2 + \frac{24 \beta^2 \zeta^2}{\mu^3 R_1^2}\Phi^2)
    \end{align}

    if we further require $K \geq \kappa$ and $s$ constant, then we have 
    \begin{align}
        F(x^{(s, R_s)}) - F(x^*) \leq c(\beta D^2 \exp(-\frac{R K}{C \kappa}) + \frac{12 \beta \sigma^2}{\mu^2 N K R} \Phi + \frac{48 \beta^2 \sigma^2}{\mu ^3 K R^2} \Phi^2 + \frac{96 \beta^2 \zeta^2}{\mu^3 R^2}\Phi^2)
    \end{align}
    for some universal constants $c, C$.
\end{proposition}

\begin{proof}
    Let $\bar{x}_{rK + k} := \frac{1}{N} \sum_{i=1}^N x^{(r)}_{i,k}$.  Then by \cite{woodworth2020minibatch} Lemma 7 under \pcref{asm:strongconvex}, \pcref{asm:grad_het}, \pcref{asm:uniform_variance}, FedAvg \pcref{algo:fedavg} under constant stepsize $\eta \leq \frac{1}{10 \beta}$,
    \begin{align}
        \E \|\bar{x}_{t+1} - x^*\|^2 &\leq (1 - \mu \eta)\E \|\bar{x}_{t} - x^*\|^2 + \frac{3 \sigma^2 \eta}{N} + 6 \beta K \eta^2(\sigma^2 + 2 K \zeta^2)
    \end{align}
    Unrolling the recursion, we get 
    \begin{align}
        \E \|\bar{x}_{T} - x^*\|^2 \leq \E \|\bar{x}_{0} - x^*\|^2 \exp(-\mu \eta T) + \frac{3 \sigma^2 \eta}{\mu N} + \frac{6 \beta K \eta^2(\sigma^2 + 2 K \zeta^2)}{\mu}
    \end{align}
    Given that $T = R'K$,
    \begin{align}
        \E \|x^{(R')} - x^*\|^2 \leq \E \|x^{(0)} - x^*\|^2 \exp(-\mu \eta R' K) + \frac{3 \sigma^2 \eta}{\mu N} + \frac{6 \beta K \eta^2(\sigma^2 + 2 K \zeta^2)}{\mu}
    \end{align}
    for any number of rounds $R'$.
    
    Let the number of rounds in the first stage be $R_1$ and the first stepsize be $\eta_1 = \eta$.  Then we have that 
    \begin{align}
        \E \|x^{(1, R_1)} - x^*\|^2 \leq \E \|x^{(0,0)} - x^*\|^2 \exp(-\mu \eta_1 R_1 K) + \frac{3 \sigma^2 \eta_1}{\mu N} + \frac{6 \beta K \eta_1^2(\sigma^2 + 2 K \zeta^2)}{\mu}
    \end{align}

    The rest of the proof follows that of \cref{thm:pl-m-sgd}.
\end{proof}
\subsection{FedAvg $\to$ SGD}
\begin{theorem}
    \label{thm:lsgd-sgd}
    Suppose we run \cref{algo:chaining} where:
    \begin{enumerate}
        \item $\ahead$ is \Lsgd \pcref{algo:fedavg} under the setting of \cref{thm:fedavgstrong}, run for $R$ rounds
        \item $\atail$ is \mbsgd \pcref{algo:ambsgd} under the setting of \cref{thm:strongsgd}, run for $R$ rounds
    \end{enumerate}
    If we additionally assume that loss queries have variance bounded by $\hat{\sigma}^2$ \pcref{asm:cost_variance}, then we have convergence rate 
    \begin{align}
        \E F(\hat{x}_2) - F(x^*) \leq (\min \{\Delta \exp(-\frac{R\sqrt{K}}{\kappa}) + \frac{\zeta^2}{2 \mu} + \frac{\sigma^2}{2\mu \sqrt{K}}, \Delta \} + \frac{4\sigma}{\sqrt{N K}}) \exp(-\frac{R}{\kappa}) + \frac{\beta \sigma^2}{\mu^2 N K R} \Phi
    \end{align}
    where $\Phi := \log(\max\{e, \frac{2 \mu^2 \Delta NKR}{\beta \sigma^2}\})$.

\end{theorem}
\begin{proof}
    After running $\ahead$ where $\ahead$ is \Lsgd under the setting of \cref{thm:fedavgstrong}, we have that 
    \begin{align}
        \E F(\hat{x}_{1/2}) - F(x^*) \leq \Delta \exp(-\frac{R\sqrt{K}}{\kappa}) + \frac{\zeta^2}{2 \mu} + \frac{\sigma^2}{2\mu \sqrt{K}}
    \end{align}
    By \cref{lemma:choosefunc}, we know that under \cref{asm:cost_variance}, we have 
    \begin{align}
        \E F(\hat{x}_1) - F(x^*) &\leq \min \{\E F(\hat{x}_{1/2}) - F(x^*), \E F(\hat{x}_{0}) - F(x^*)\} + \frac{4\sigma}{\sqrt{N K}} \\
        &\leq \min \{\Delta \exp(-\frac{R\sqrt{K}}{\kappa}) + \frac{\zeta^2}{2 \mu} + \frac{\sigma^2}{2\mu \sqrt{K}}, \Delta \} + \frac{4\sigma}{\sqrt{N K}}
    \end{align}
    Now we run $\atail$ as \mbsgd \pcref{algo:mbsgd} under the setting of \cref{thm:strongsgd} using $\hat{x}_1$ is the initialization, which gives
    \begin{align}
        \E F(\hat{x}_2) - F(x^*) \leq (\E F(\hat{x}_1) - F(x^*)) \exp(-\frac{R}{\kappa}) + \frac{\beta \sigma^2}{\mu^2 N K R} \Phi
    \end{align}
    Where $\Phi := \log(\max\{e, \frac{2 \mu^2 \Delta NKR}{\beta \sigma^2}\})$.
    which gives the convergence rate
    \begin{align}
        \E F(\hat{x}_2) - F(x^*) \leq (\min \{\Delta \exp(-\frac{R\sqrt{K}}{\kappa}) + \frac{\zeta^2}{2 \mu} + \frac{\sigma^2}{2\mu \sqrt{K}}, \Delta \} + \frac{4\sigma}{\sqrt{N K}}) \exp(-\frac{R}{\kappa}) + \frac{\beta \sigma^2}{\mu^2 N K R} \Phi
    \end{align}

\end{proof}
\subsection{\lsgd $\to$ \asg}
\begin{theorem}
    \label{thm:lsgd-asg}
    Suppose we run \cref{algo:chaining} where:
    \begin{enumerate}
        \item $\ahead$ is \Lsgd \pcref{algo:fedavg} under the setting of \cref{thm:fedavgstrong}, run for $R$ rounds
        \item $\atail$ is \asg\pcref{algo:ambsgd} under the setting of \cref{thm:appasg}, run for $R$ rounds
    \end{enumerate}
    If we additionally assume that loss queries have variance bounded by $\sigma^2$ \pcref{asm:cost_variance}, this gives the convergence rate
    \begin{align}
        \E F(\hat{x}_2) - F(x^*) &\leq 2 (\min \{\Delta \exp(-\frac{R\sqrt{K}}{\kappa}) + \frac{\zeta^2}{2 \mu} + \frac{\sigma^2}{2\mu \sqrt{K}}, \Delta \} + \frac{4\sigma}{\sqrt{N K}}) \exp(- \frac{R}{\sqrt{\kappa}}) \\
        & \ \ \ \ +  \frac{\sigma^2}{\mu N K R} \Phi^{1/2} + \frac{\beta \sigma^2}{\mu^2 N K R^3} \Phi^{3/2}
    \end{align}
    where
    \begin{align}
		\Phi = \log(\max\{e, \min \{\frac{2 \Delta  \mu N K R}{\sigma^2}, \frac{2 \Delta \mu^2  N K R^3  }{\beta \sigma^2}\}\})
	\end{align}
\end{theorem}
\begin{proof}
    After running $\ahead$ where $\ahead$ is \Lsgd under the setting of \cref{thm:fedavgstrong}, we have that 
    \begin{align}
        \E F(\hat{x}_{1/2}) - F(x^*) \leq \Delta \exp(-\frac{R\sqrt{K}}{\kappa}) + \frac{\zeta^2}{2 \mu} + \frac{\sigma^2}{2\mu \sqrt{K}}
    \end{align}
    By \cref{lemma:choosefunc}, we know that under \cref{asm:cost_variance}, we have 
    \begin{align}
        \E F(\hat{x}_1) - F(x^*) &\leq \min \{\E F(\hat{x}_{1/2}) - F(x^*), \E F(\hat{x}_{0}) - F(x^*)\} + \frac{4\sigma}{\sqrt{N K}} \\
        &\leq \min \{\Delta \exp(-\frac{R\sqrt{K}}{\kappa}) + \frac{\zeta^2}{2 \mu} + \frac{\sigma^2}{2\mu \sqrt{K}}, \Delta \} + \frac{4\sigma}{\sqrt{N K}}
    \end{align}
    Now we run $\atail$ as \asg \pcref{algo:ambsgd} under the setting of \cref{thm:appasg} using $\hat{x}_1$ is the initialization, which gives
    
    \begin{align}
        \E F(\hat{x}_1) - F(x^*) \leq 2 (\E F(\hat{x}_1) - F(x^*)) \exp(- \frac{R}{\sqrt{\kappa}}) +  \frac{\sigma^2}{\mu N K R} \Phi^{1/2} + \frac{\beta \sigma^2}{\mu^2 N K R^3} \Phi^{3/2}
    \end{align}
    where 
    \begin{align}
		\Phi = \log(\max\{e, \min \{\frac{2 \Delta  \mu N K R}{\sigma^2}, \frac{2 \Delta \mu^2  N K R^3  }{\beta \sigma^2}\}\})
	\end{align}
    which gives the convergence rate
    \begin{align}
        \E F(\hat{x}_2) - F(x^*) &\leq 2 (\min \{\Delta \exp(-\frac{R\sqrt{K}}{\kappa}) + \frac{\zeta^2}{2 \mu} + \frac{\sigma^2}{2\mu \sqrt{K}}, \Delta \} + \frac{4\sigma}{\sqrt{N K}}) \exp(- \frac{R}{\sqrt{\kappa}}) \\
        & \ \ \ \ +  \frac{\sigma^2}{\mu N K R} \Phi^{1/2} + \frac{\beta \sigma^2}{\mu^2 N K R^3} \Phi^{3/2}
    \end{align}
\end{proof}
\subsection{M-\Lsgd $\to$ M-\mbsgd}
\begin{theorem}
    \label{thm:strong-mlsgd-msgd}
    Suppose we run \cref{algo:chaining} where:
    \begin{enumerate}
        \item $\ahead$ is M-\Lsgd \pcref{algo:m-lsgd} under the setting of \cref{thm:mfedavg}, run for $R$ rounds
        \item $\atail$ is M-\mbsgd \pcref{algo:m-mbsgd} under the setting of \cref{thm:pl-m-sgd}, run for $R$ rounds
    \end{enumerate}
    If we additionally assume that loss queries have variance bounded by $\sigma^2$ \pcref{asm:cost_variance}, then we have convergence rate 
    \begin{align}
        & \ \ \E F(\hat{x}_2) - F(x^*) \\
        &\leq c'( c(\exp(- \frac{R}{C' \kappa})(\min \{(\beta D^2 \exp(-\frac{R K}{C \kappa}) + \frac{12 \beta \sigma^2}{\mu^2 N K R} \Phi + \frac{48 \beta^2 \sigma^2}{\mu ^3 K R^2} \Phi^2 + \frac{96 \beta^2 \zeta^2}{\mu^3 R^2}\Phi^2), \Delta \} + \frac{4\sigma}{\sqrt{N K}})  \\
        & \ \ \ + \frac{\beta \sigma^2}{\mu^2 N K R} \Phi')
    \end{align}
    Where $\Phi = \log(\max \{e, \min \{\frac{\mu^2 D^2 N K^2 R_1}{3 \sigma^2}, \frac{\mu^3 D^2 K R_1^2}{6 \beta  (\sigma^2 + 2 K \zeta^2)})$, $\Phi' = \log(\max\{e, \frac{2 \mu^2 \Delta NKR}{\beta \sigma^2}\})$
    and $c,c',C, C'$ are absolute constants.
\end{theorem}
\begin{proof}
    The proof follows that of \cref{thm:m-lsgd-asg}.
\end{proof}
\subsection{M-\lsgd $\to$ M-\asg}
\begin{theorem}
    \label{thm:m-lsgd-asg}
    Suppose we run \cref{algo:chaining} where:
    \begin{enumerate}
        \item $\ahead$ is M-\Lsgd \pcref{algo:m-lsgd} under the setting of \cref{thm:mfedavg}, run for $R$ rounds
        \item $\atail$ is M-\asg \pcref{algo:m-ambsgd} under the setting of Theorem 3.6 of \cite{aybat2019universally}, run for $R$ rounds
    \end{enumerate}
    If we additionally assume that loss queries have variance bounded by $\sigma^2$ \pcref{asm:cost_variance}, then we have convergence rate
    \begin{align}
        &\E F(\hat{x}_2) - F(x^*) \leq \\
        &c(\exp(- \frac{R}{2 \sqrt{\kappa}})(\min \{(\beta D^2 \exp(-\frac{R K}{20 \kappa}) + \frac{12 \beta \sigma^2}{\mu^2 N K R} \Phi + \frac{48 \beta^2 \sigma^2}{\mu ^3 K R^2} \Phi^2 + \frac{96 \beta^2 \zeta^2}{\mu^3 R^2}\Phi^2), \Delta \} + \frac{4\sigma}{\sqrt{N K}}) + \frac{\sigma^2}{\mu N K R})
    \end{align}
    where
    \begin{align}
        \Phi = \log(\max \{e, \min \{\frac{\mu^2 D^2 N K^2 R_1}{3 \sigma^2}, \frac{\mu^3 D^2 K R_1^2}{6 \beta  (\sigma^2 + 2 K \zeta^2)})
    \end{align}
    $R_1$ being the number of rounds in the first stage of M-\lsgd, and $c$ is some universal constant.
\end{theorem}
\begin{proof}
    After running $\ahead$ where $\ahead$ is M-\Lsgd under the setting of \cref{thm:mfedavg}, we have that 
    \begin{align}
        \E F(\hat{x}_{1/2}) - F(x^*) \leq c(\beta D^2 \exp(-\frac{R K}{20 \kappa}) + \frac{12 \beta \sigma^2}{\mu^2 N K R} \Phi + \frac{48 \beta^2 \sigma^2}{\mu ^3 K R^2} \Phi^2 + \frac{96 \beta^2 \zeta^2}{\mu^3 R^2}\Phi^2)
    \end{align}
    where 
    \begin{align}
        \Phi = \log(\max \{e, \min \{\frac{\mu^2 D^2 N K R_1}{3 \sigma^2}, \frac{\mu^3 D^2 K R_1^2}{6 \beta  (\sigma^2 + 2 K \zeta^2)})
    \end{align}
    $R_1$ being the number of rounds in the first stage of M-\lsgd.
    By \cref{lemma:choosefunc}, we know that under \cref{asm:cost_variance}, we have 
    \begin{align}
        \E F(\hat{x}_1) - F(x^*) &\leq \min \{\E F(\hat{x}_{1/2}) - F(x^*), \E F(\hat{x}_{0}) - F(x^*)\} + \frac{4\sigma}{\sqrt{N K}} \\
        &\leq \min \{c(\beta D^2 \exp(-\frac{R K}{20 \kappa}) + \frac{12 \beta \sigma^2}{\mu^2 N K R} \Phi + \frac{48 \beta^2 \sigma^2}{\mu ^3 K R^2} \Phi^2 + \frac{96 \beta^2 \zeta^2}{\mu^3 R^2}\Phi^2), \Delta \} + \frac{4\sigma}{\sqrt{N K}}
    \end{align}
    Now we run $\atail$ as M-\asg \pcref{algo:m-ambsgd} under the setting of Theorem 3.6 of \cite{aybat2019universally} using $\hat{x}_1$ is the initialization, which gives
    
    \begin{align}
        \E F(\hat{x}_2) - F(x^*) \leq c'(\exp(- \frac{R}{2 \sqrt{\kappa}})(\E F(\hat{x}_1) - F(x^*)) + \frac{\sigma^2}{\mu N K R})
    \end{align}
    which gives the convergence rate
    \begin{align}
        &\E F(\hat{x}_2) - F(x^*) \leq \\
        &c'(\exp(- \frac{R}{2 \sqrt{\kappa}})(\min \{c(\beta D^2 \exp(-\frac{R K}{20 \kappa}) + \frac{12 \beta \sigma^2}{\mu^2 N K R} \Phi + \frac{48 \beta^2 \sigma^2}{\mu ^3 K R^2} \Phi^2 + \frac{96 \beta^2 \zeta^2}{\mu^3 R^2}\Phi^2), \Delta \} + \frac{4\sigma}{\sqrt{N K}}) + \frac{\sigma^2}{\mu N K R})
    \end{align}
\end{proof}
